# Supplementary material for: A General Framework for Multivariate Functional Principal Component Analysis of Amplitude and Phase Variation
Source: arXiv:1810.13321 source file (2018-10-31)
Supplement: Supplementary file 1 [file seisPlots_tw_smooth_rawPCA.pdf]

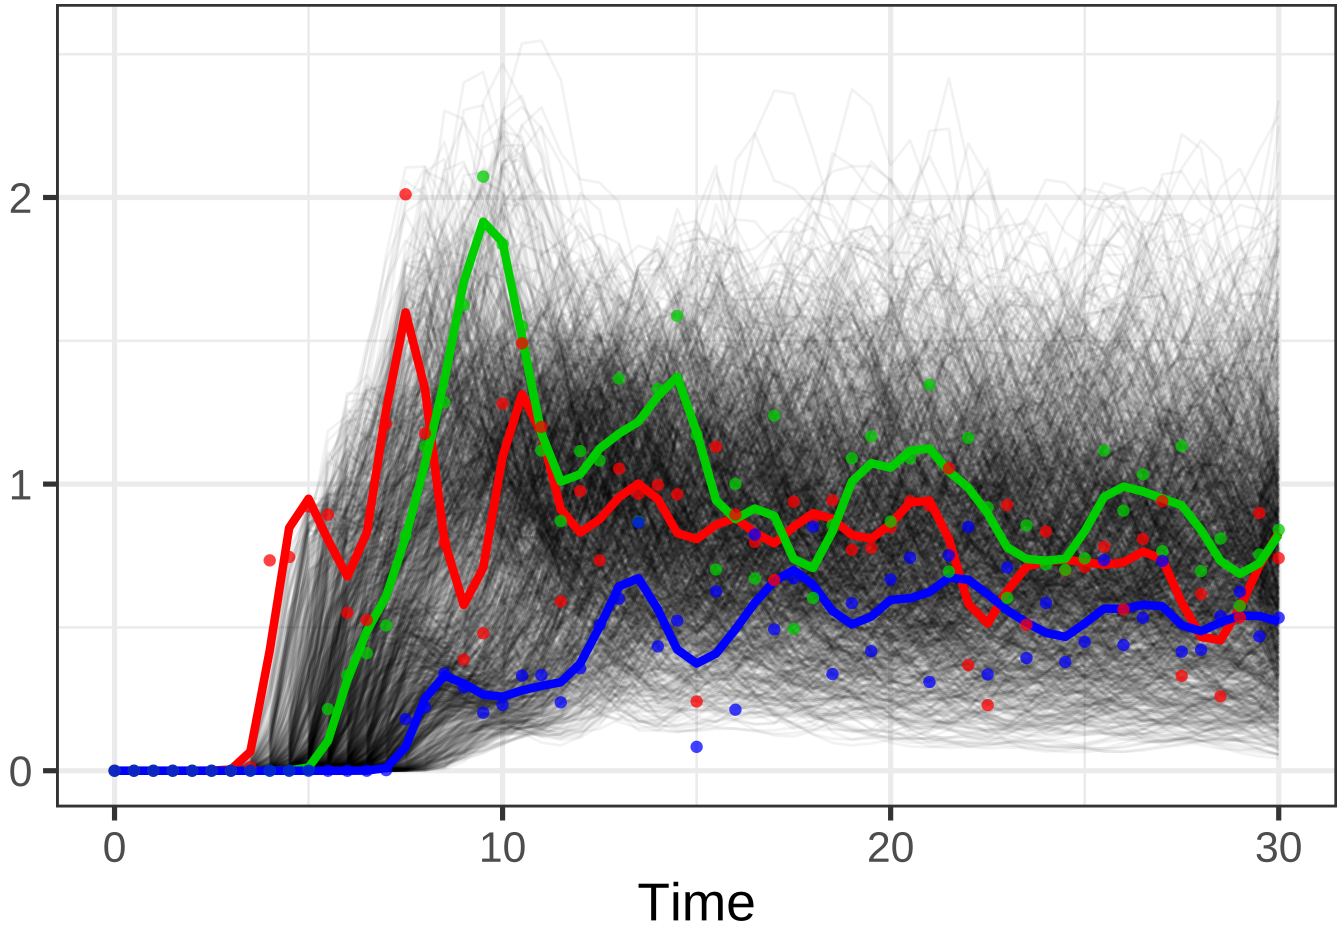

2
1
0
0
10
20
30
Time

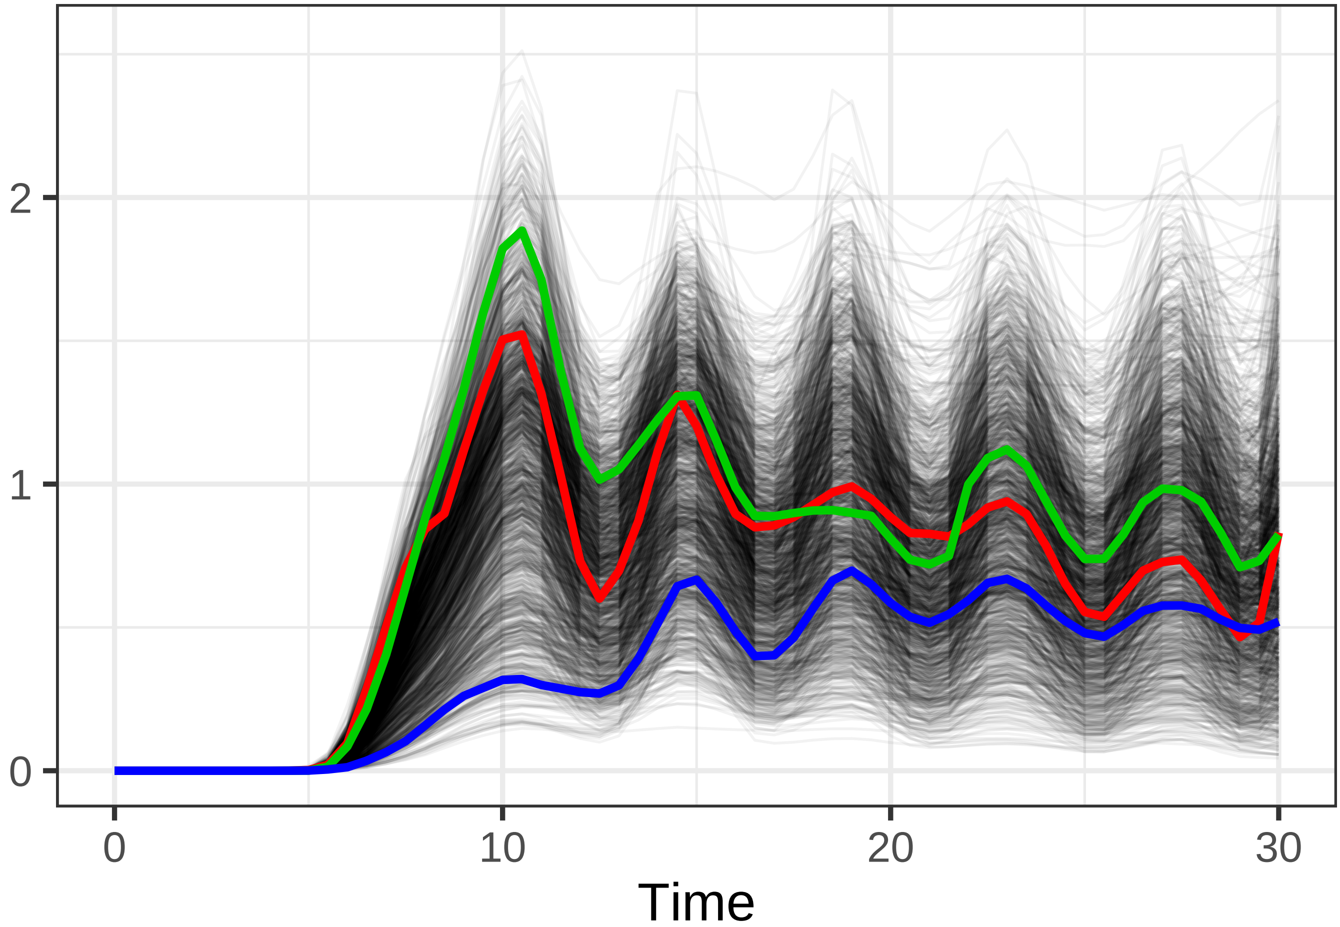
0
1
2
0
10
20
30
Time

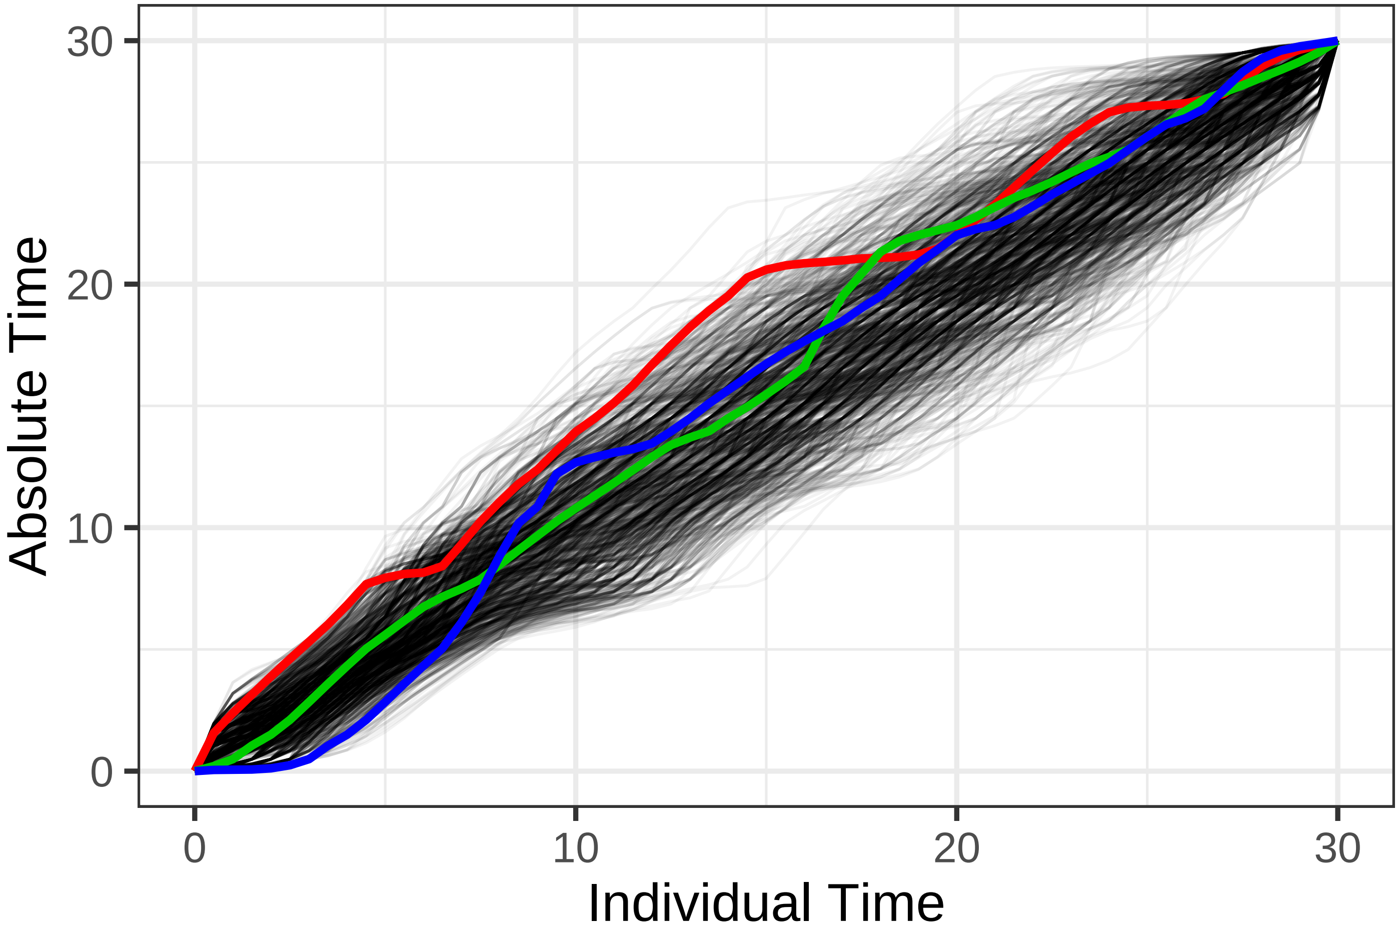

Absolute Time
Individual Time
0
10
20
30
0
10
20
30

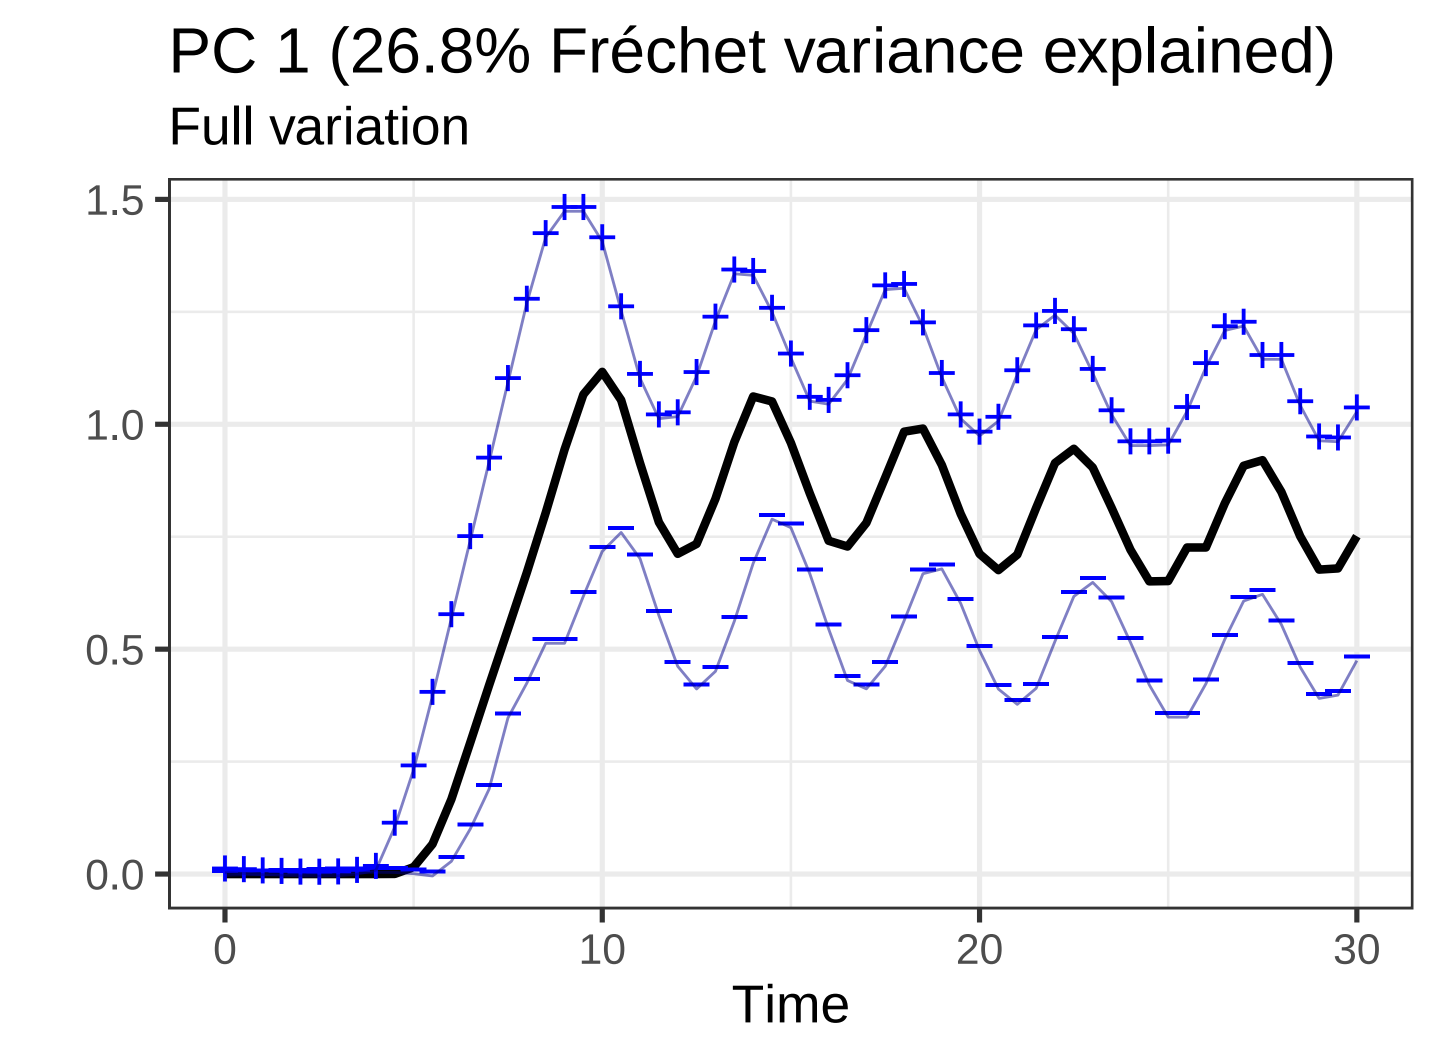
PC 1 (26.8% Fréchet variance explained)
Full variation
1.5
1.0
0.5
0.0
0
10
20
30
Time

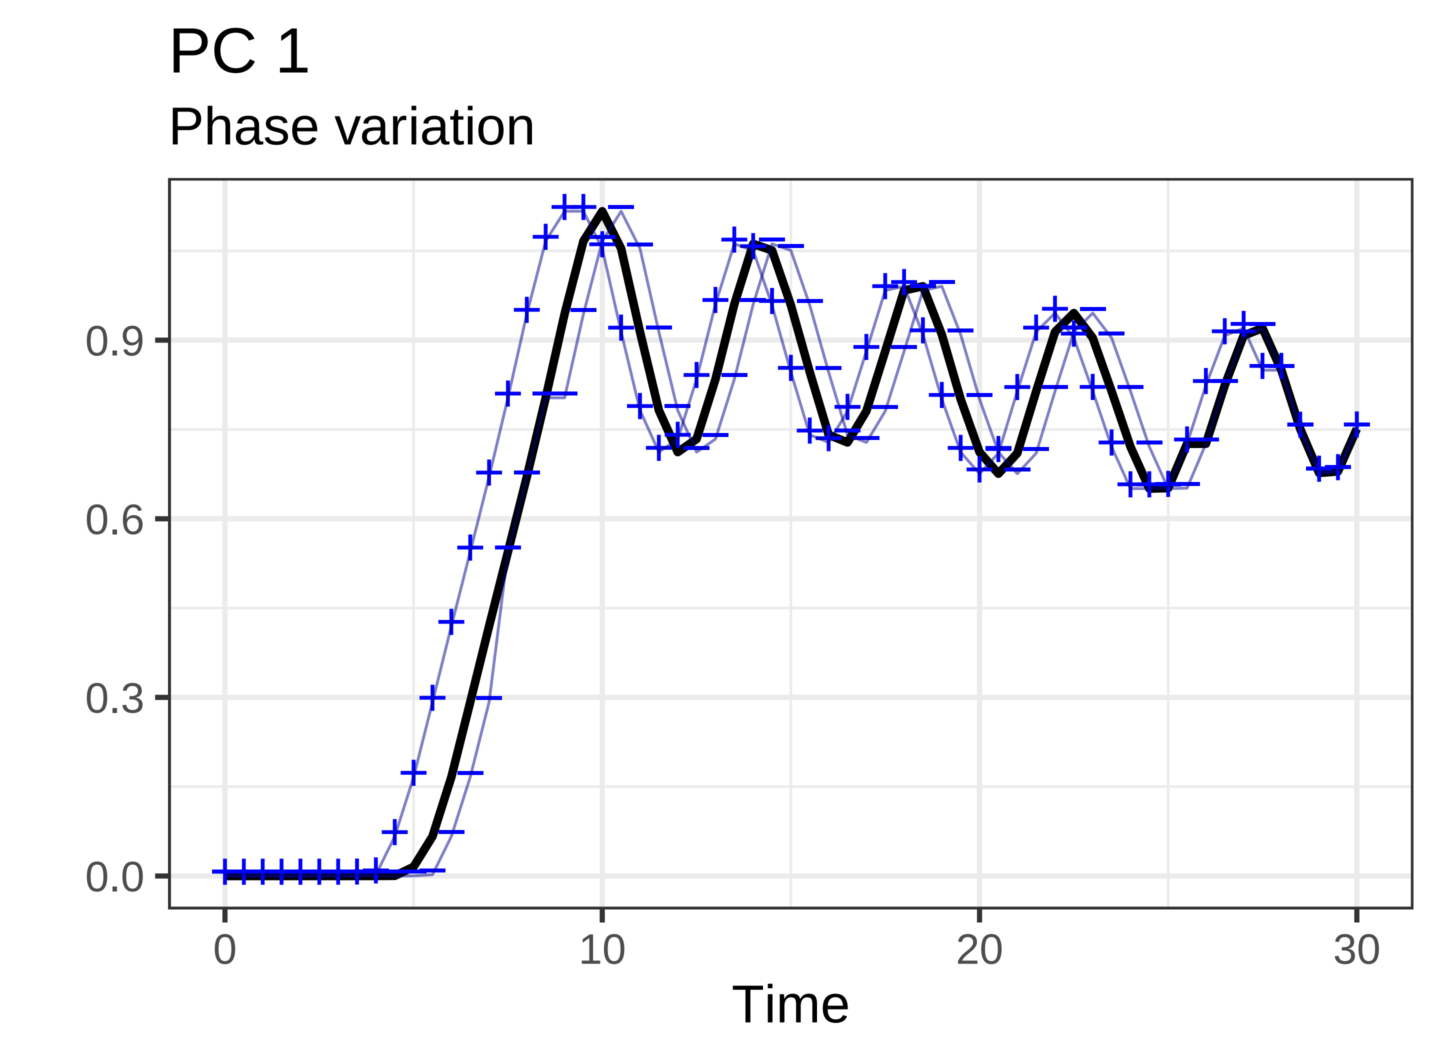
PC 1
Phase variation
0.0
0.3
0.6
0.9
0
10
20
30
Time

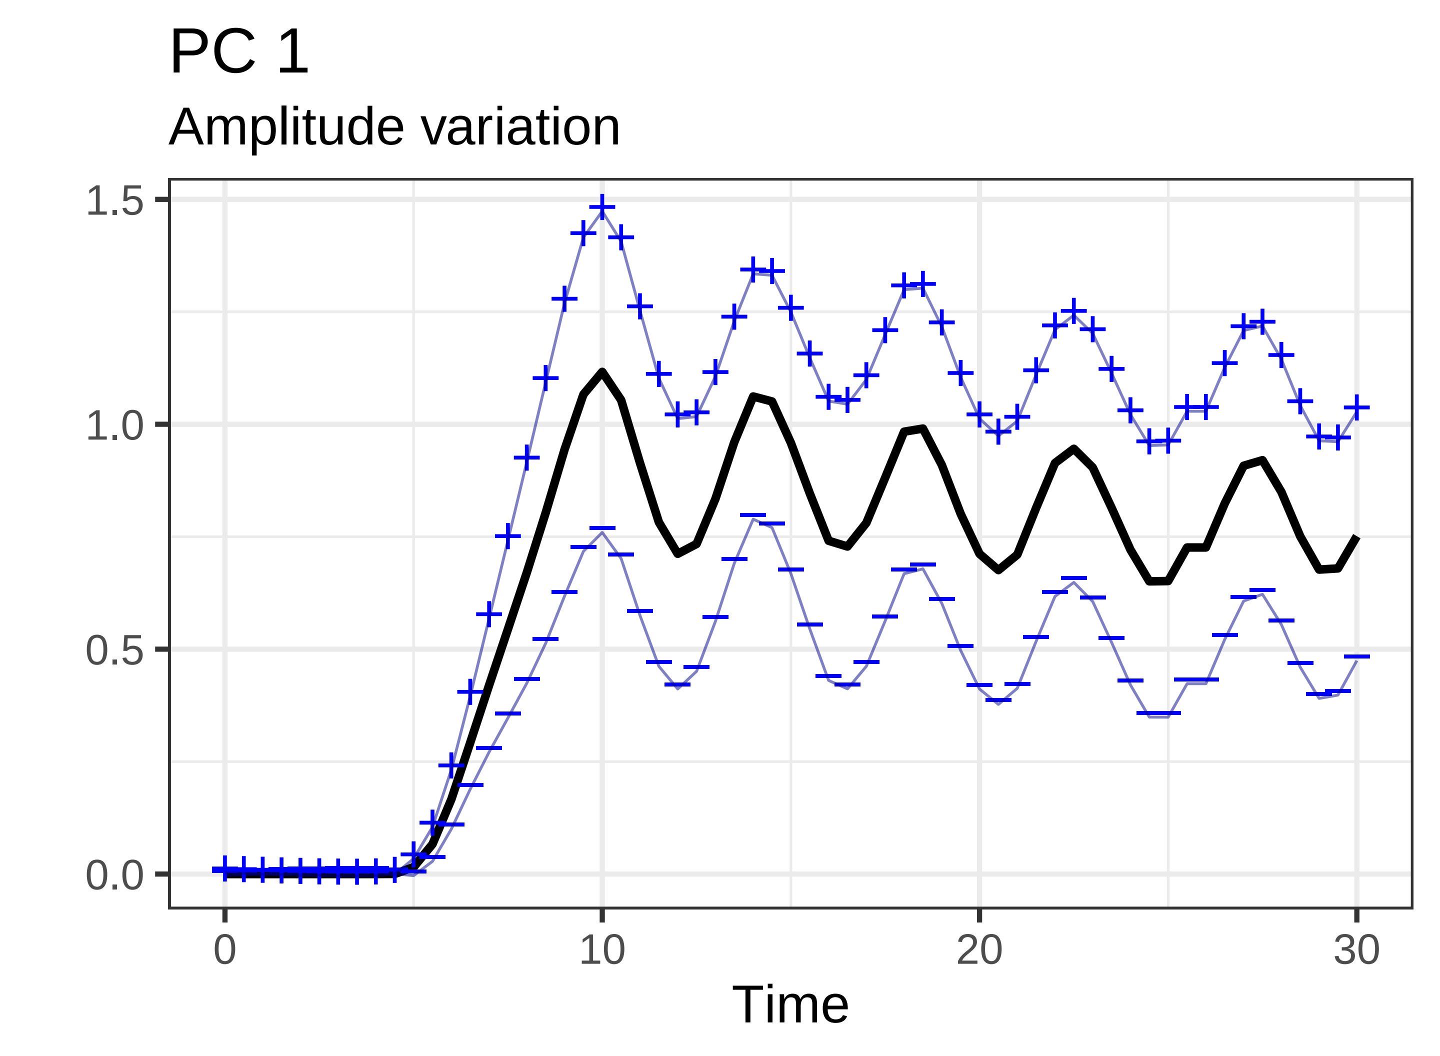

PC 1
Amplitude variation
1.5
1.0
0.5
0.0
0
10
20
30
Time

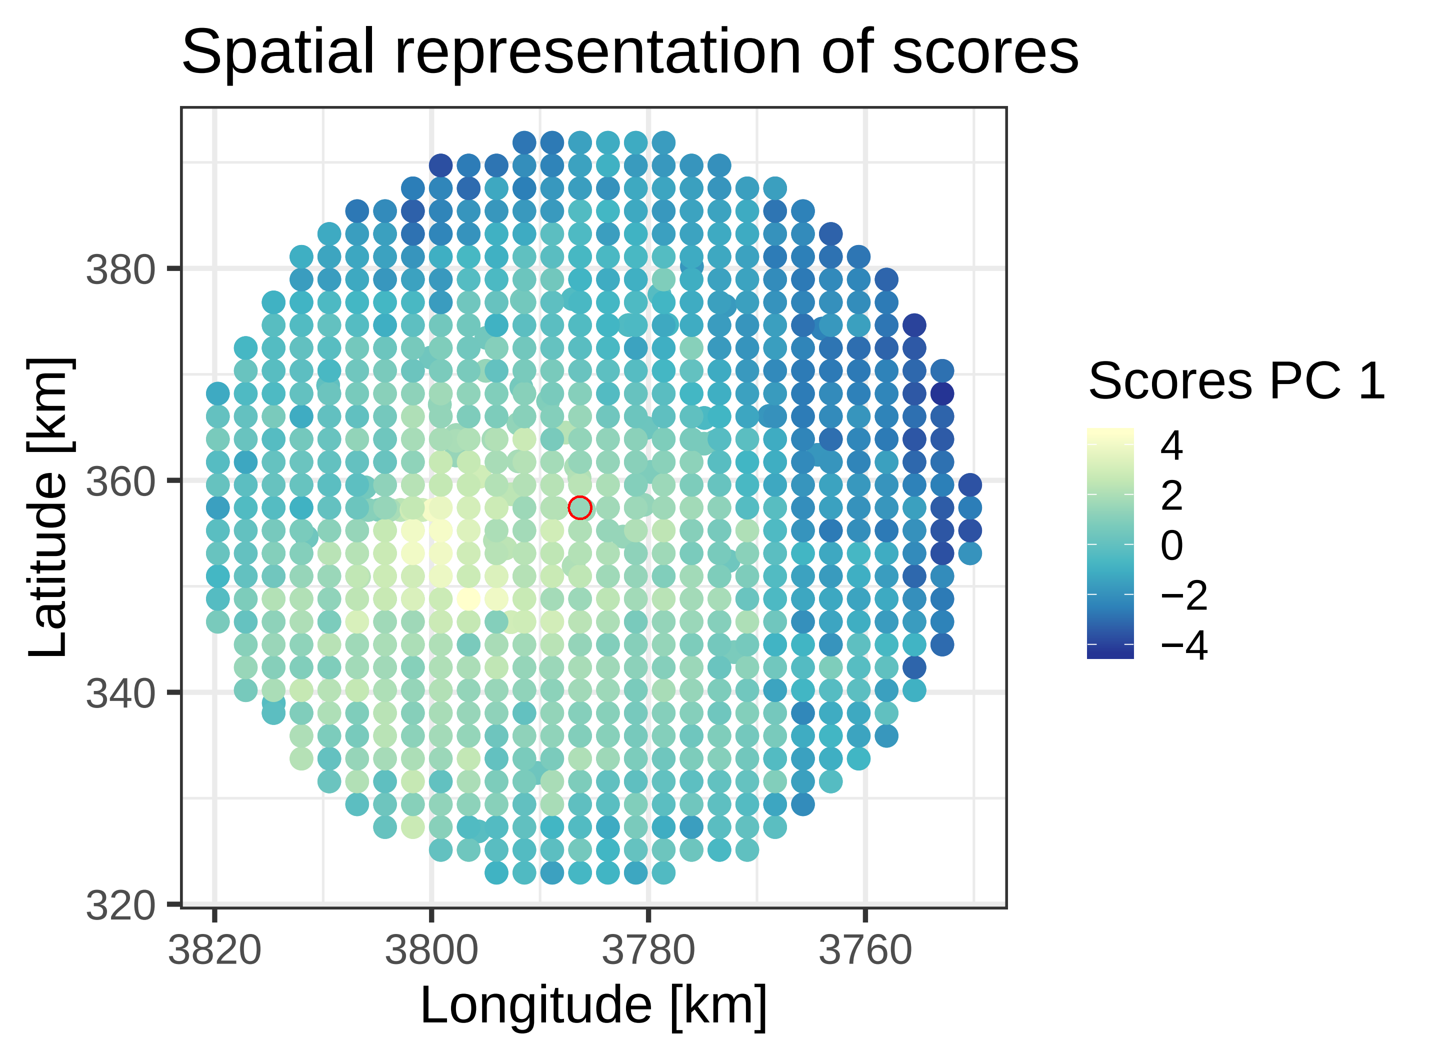

Spatial representation of scores
Latitude [km]
Longitude [km]
380
360
340
320
3820
3800
3780
3760
Scores PC 1
4
2
0
−2
−4

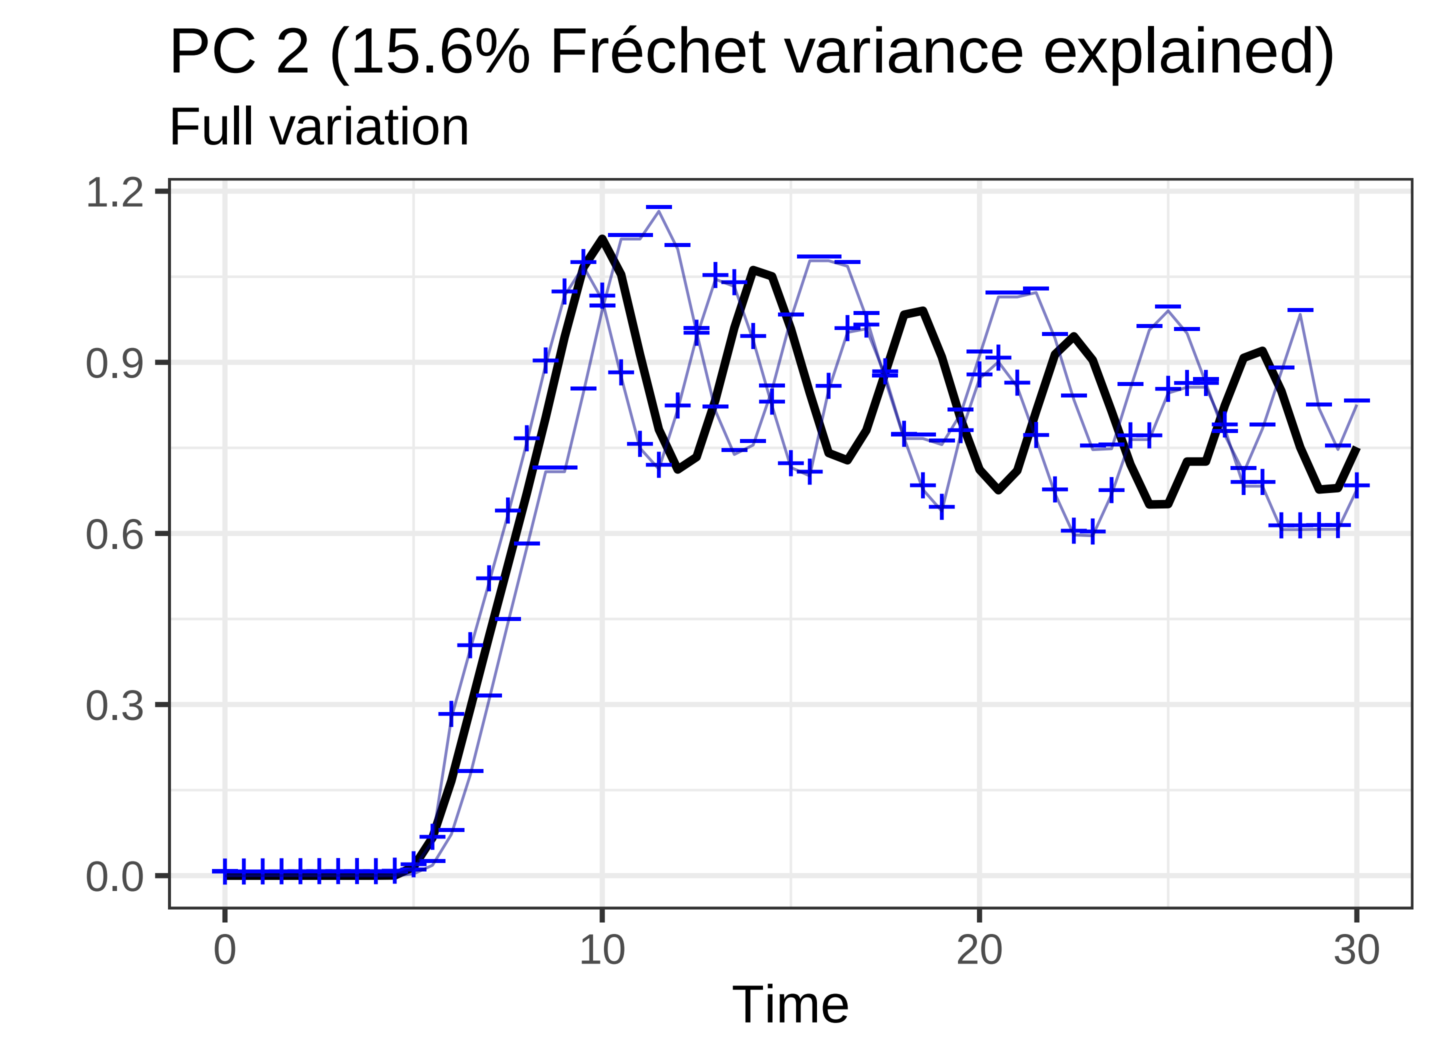

PC 2 (15.6% Fréchet variance explained)
Full variation
1.2
0.9
0.6
0.3
0.0
0
10
20
30
Time

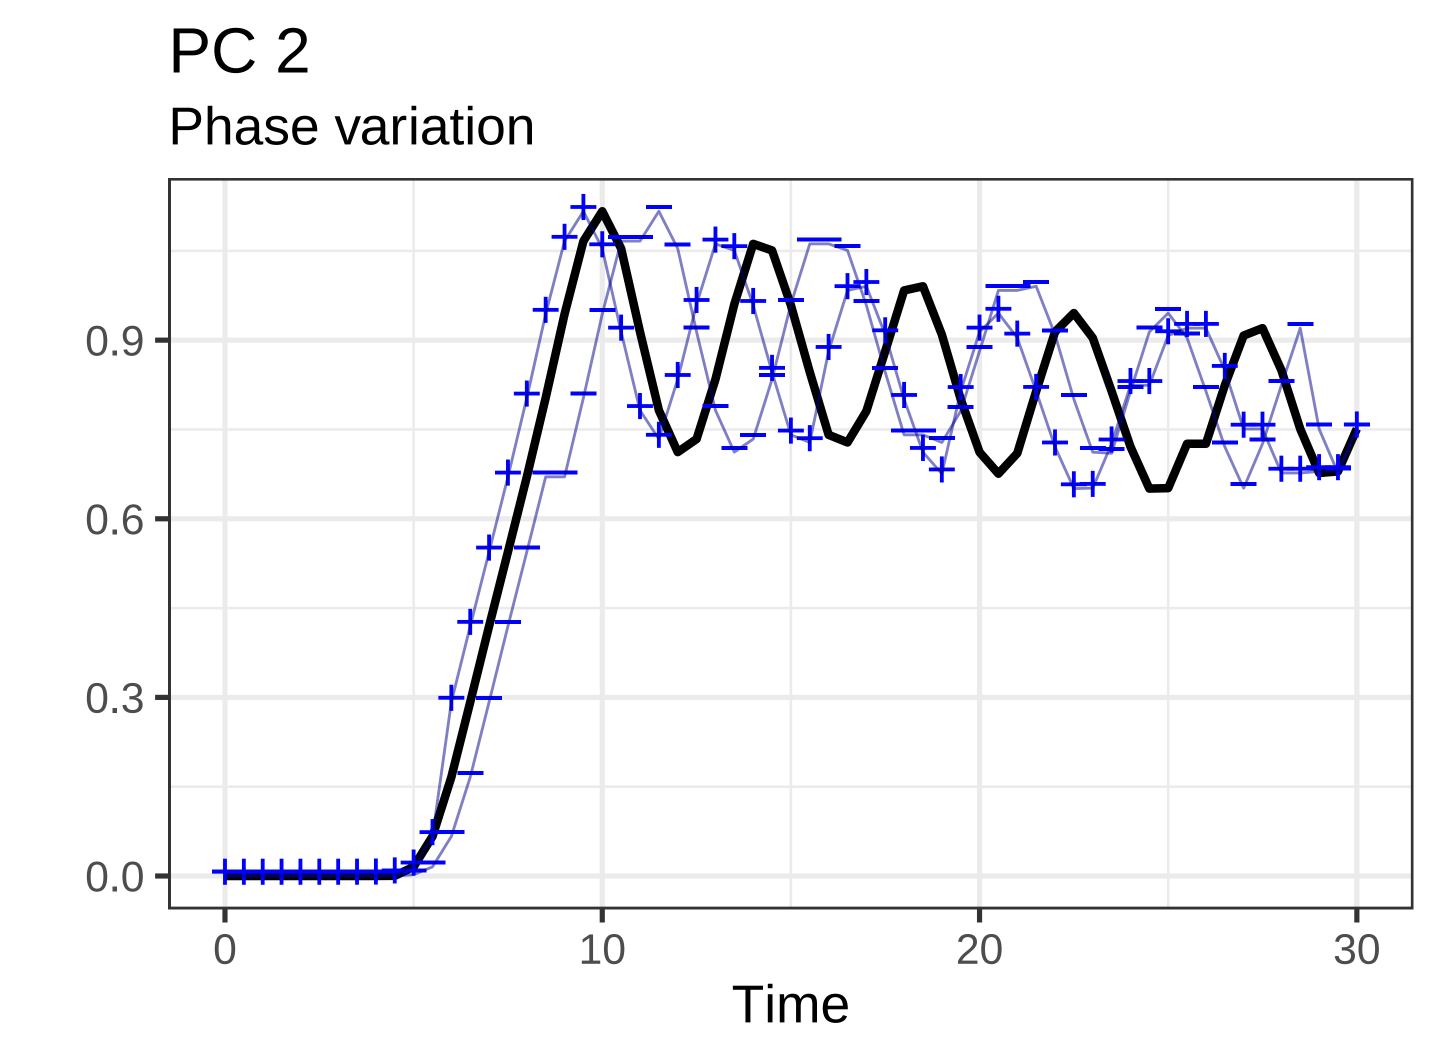

PC 2
Phase variation
0.0
0.3
0.6
0.9
0
10
20
30
Time

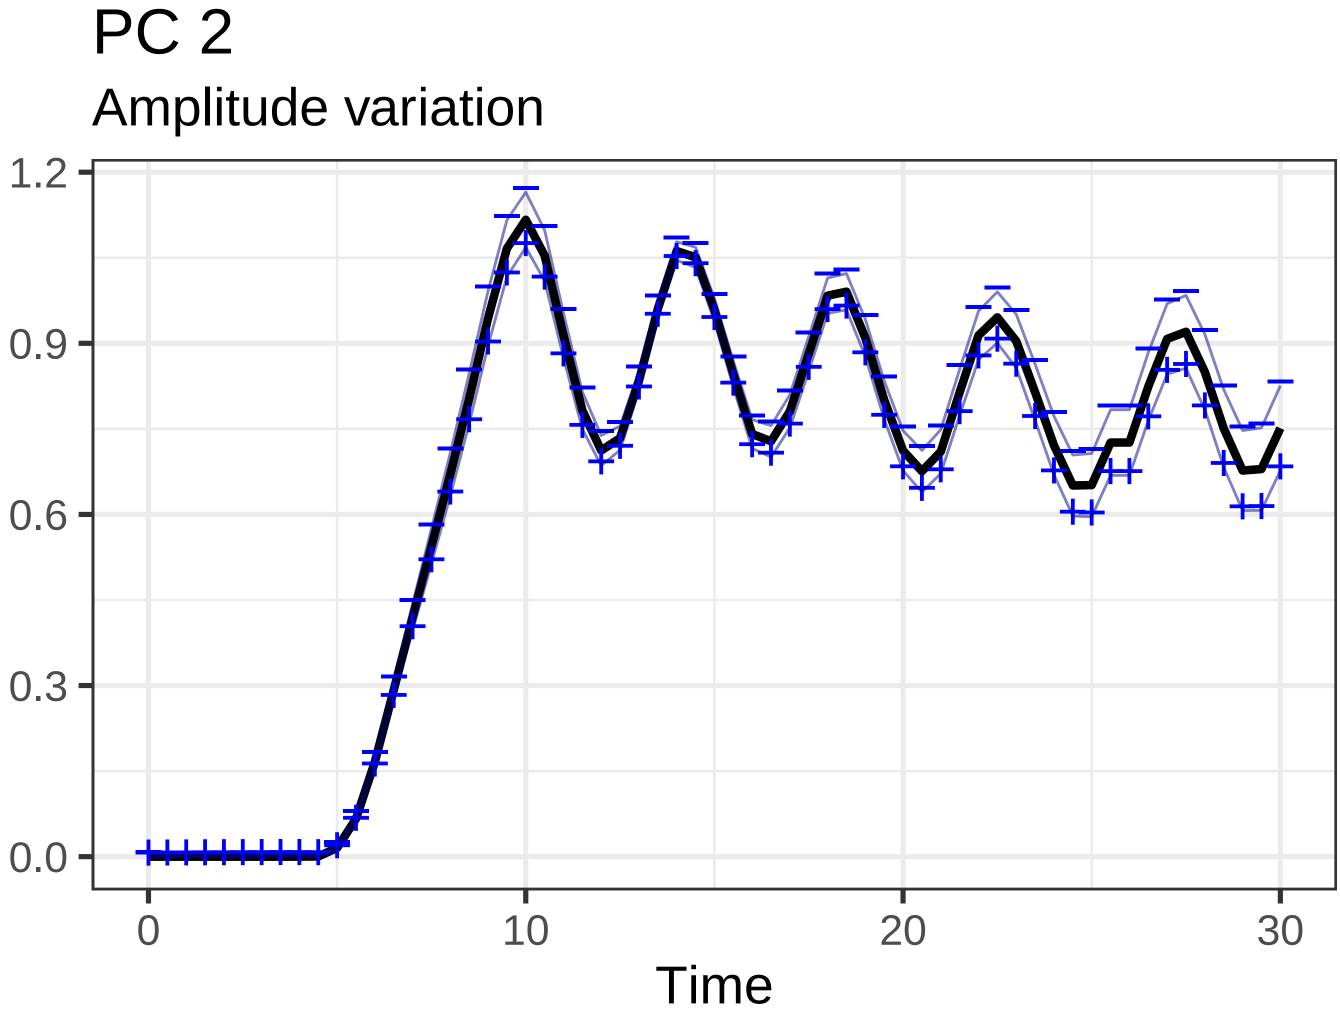

PC 2
Amplitude variation
1.2
0.9
0.6
0.3
0.0
0
10
20
30
Time

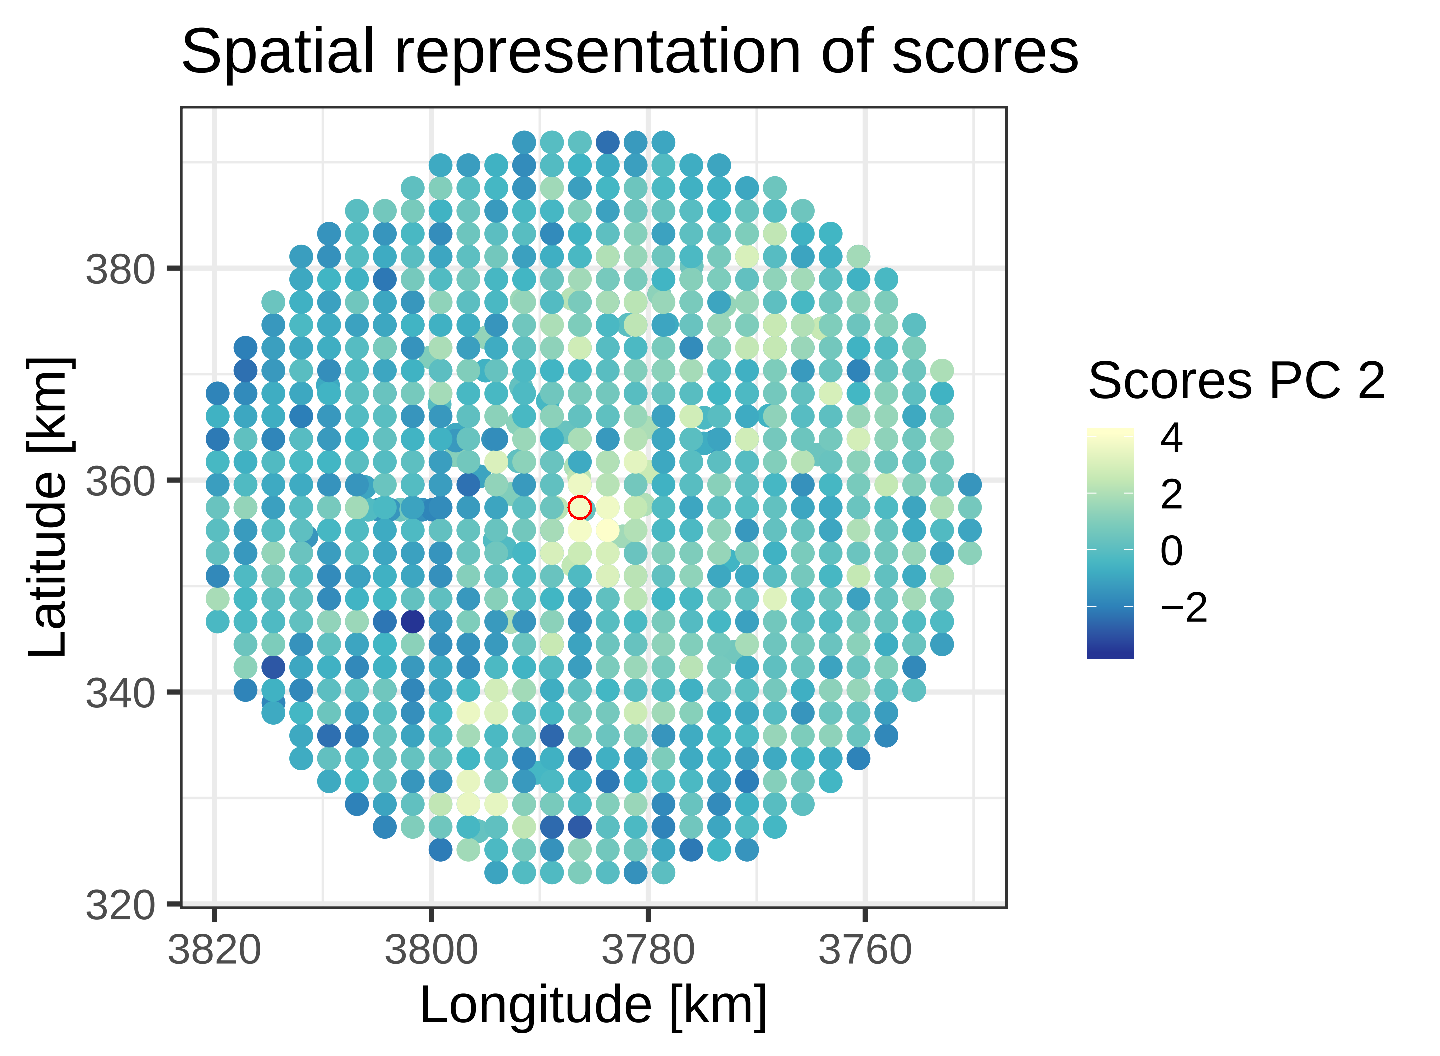
Spatial representation of scores
Latitude [km]
380
360
340
320
3820
3800
3780
3760
Longitude [km]
Scores PC 2
4
2
0
−2

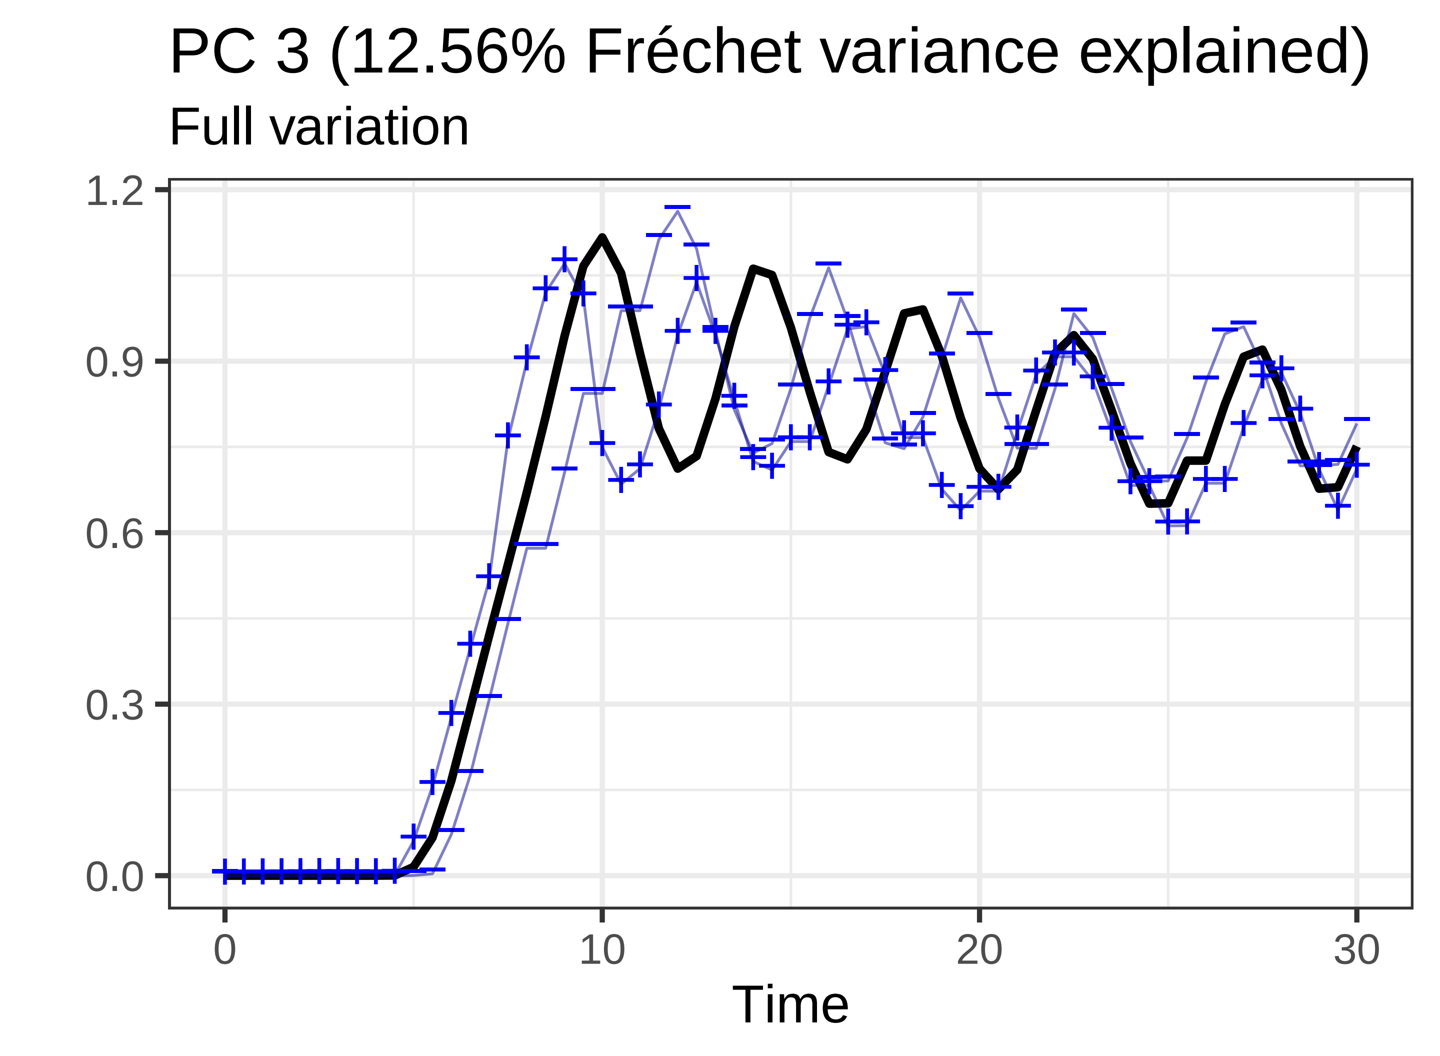

PC 3 (12.56% Fréchet variance explained)
Full variation
1.2
0.9
0.6
0.3
0.0
0
10
20
30
Time

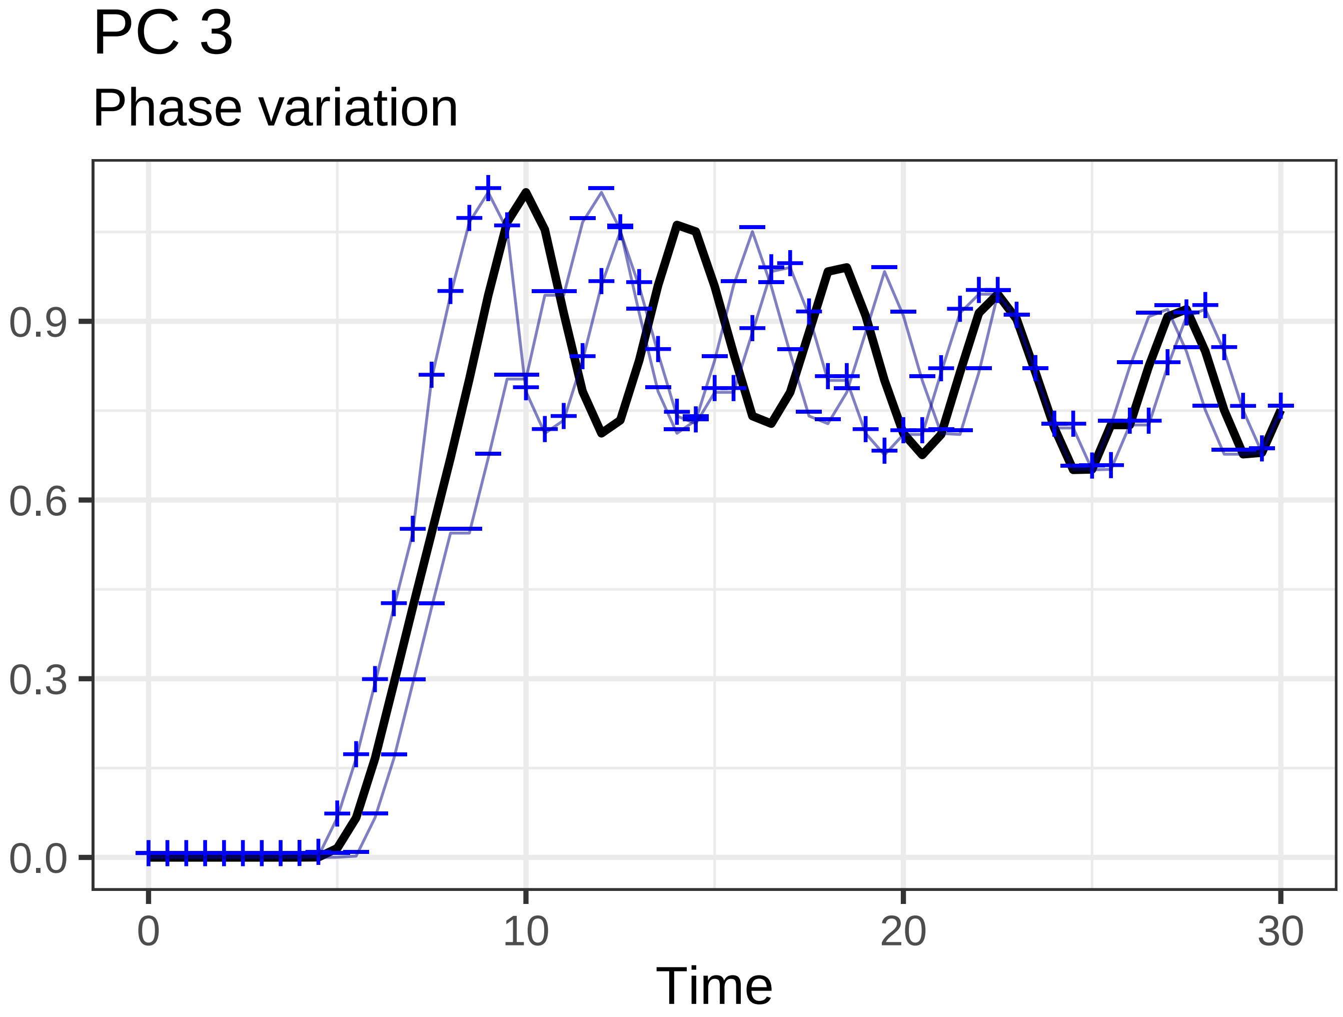

PC 3
Phase variation
0.0
0.3
0.6
0.9
0
10
20
30
Time

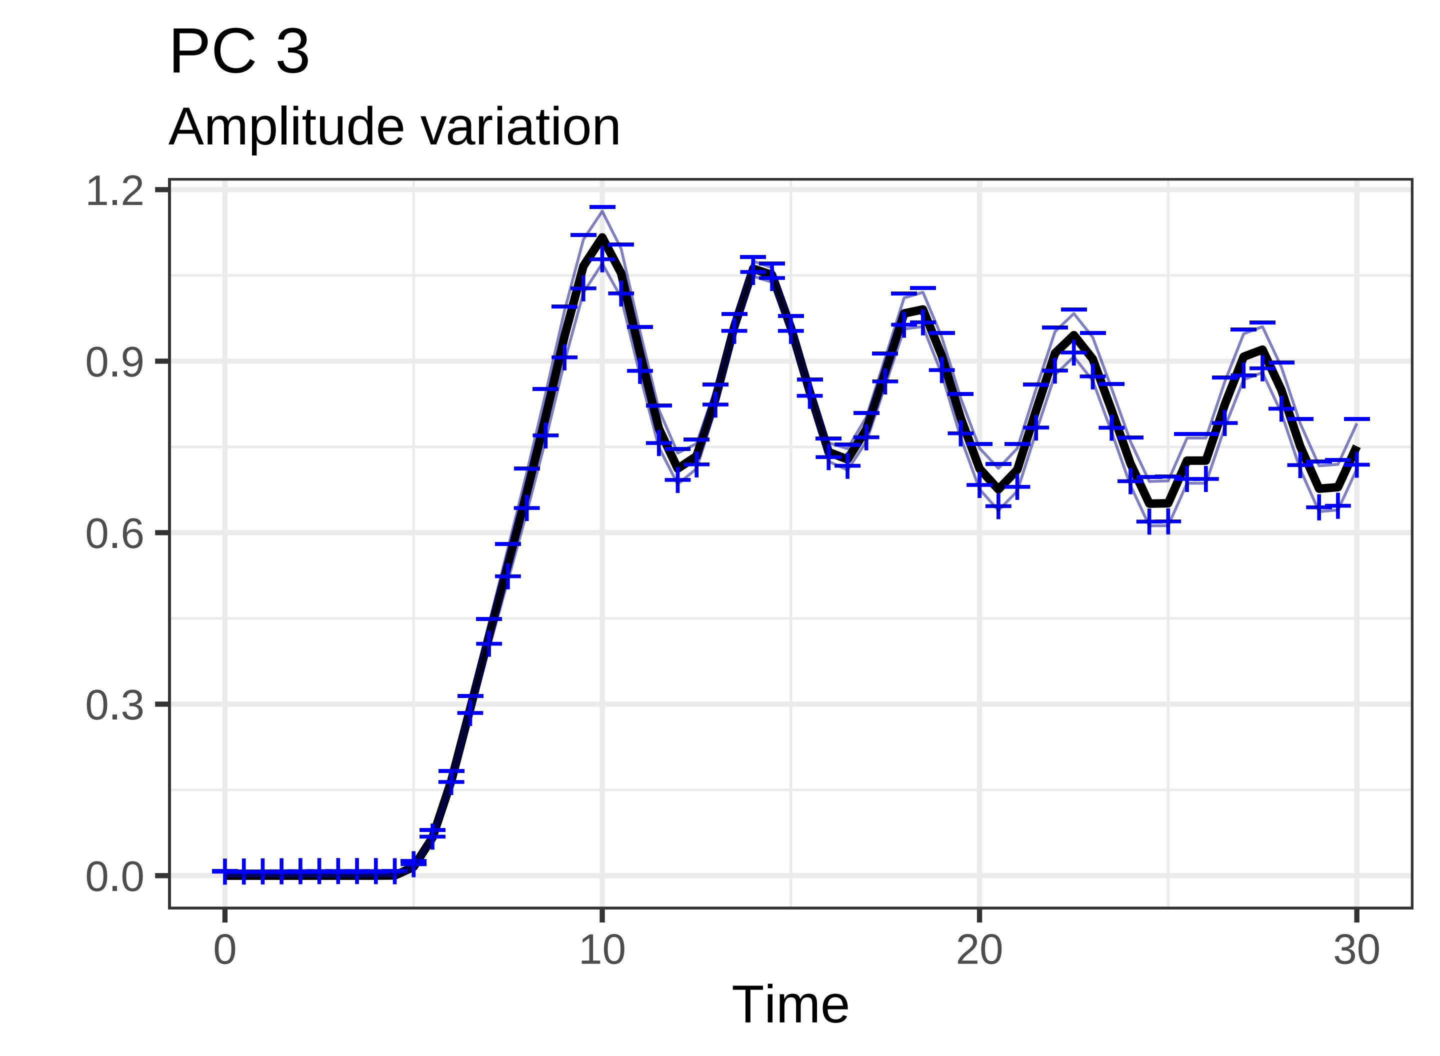

PC 3
Amplitude variation
1.2
0.9
0.6
0.3
0.0
0
10
20
30
Time

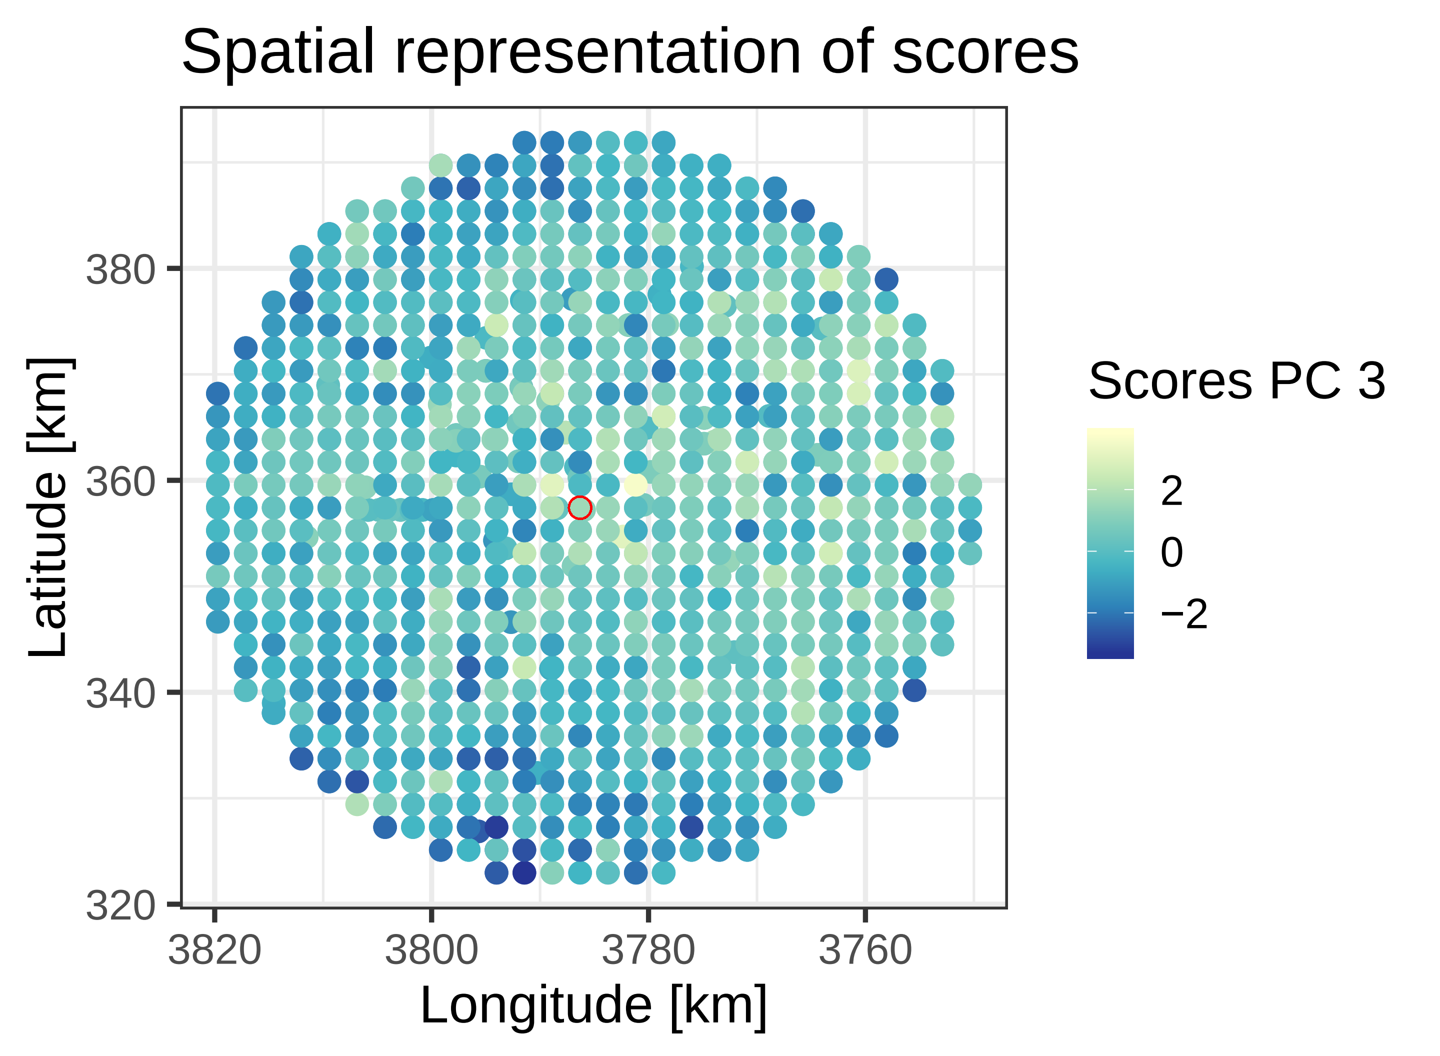

Spatial representation of scores
Latitude [km]
380
360
340
320
3820
3800
3780
3760
Longitude [km]
Scores PC 3
2
0
−2

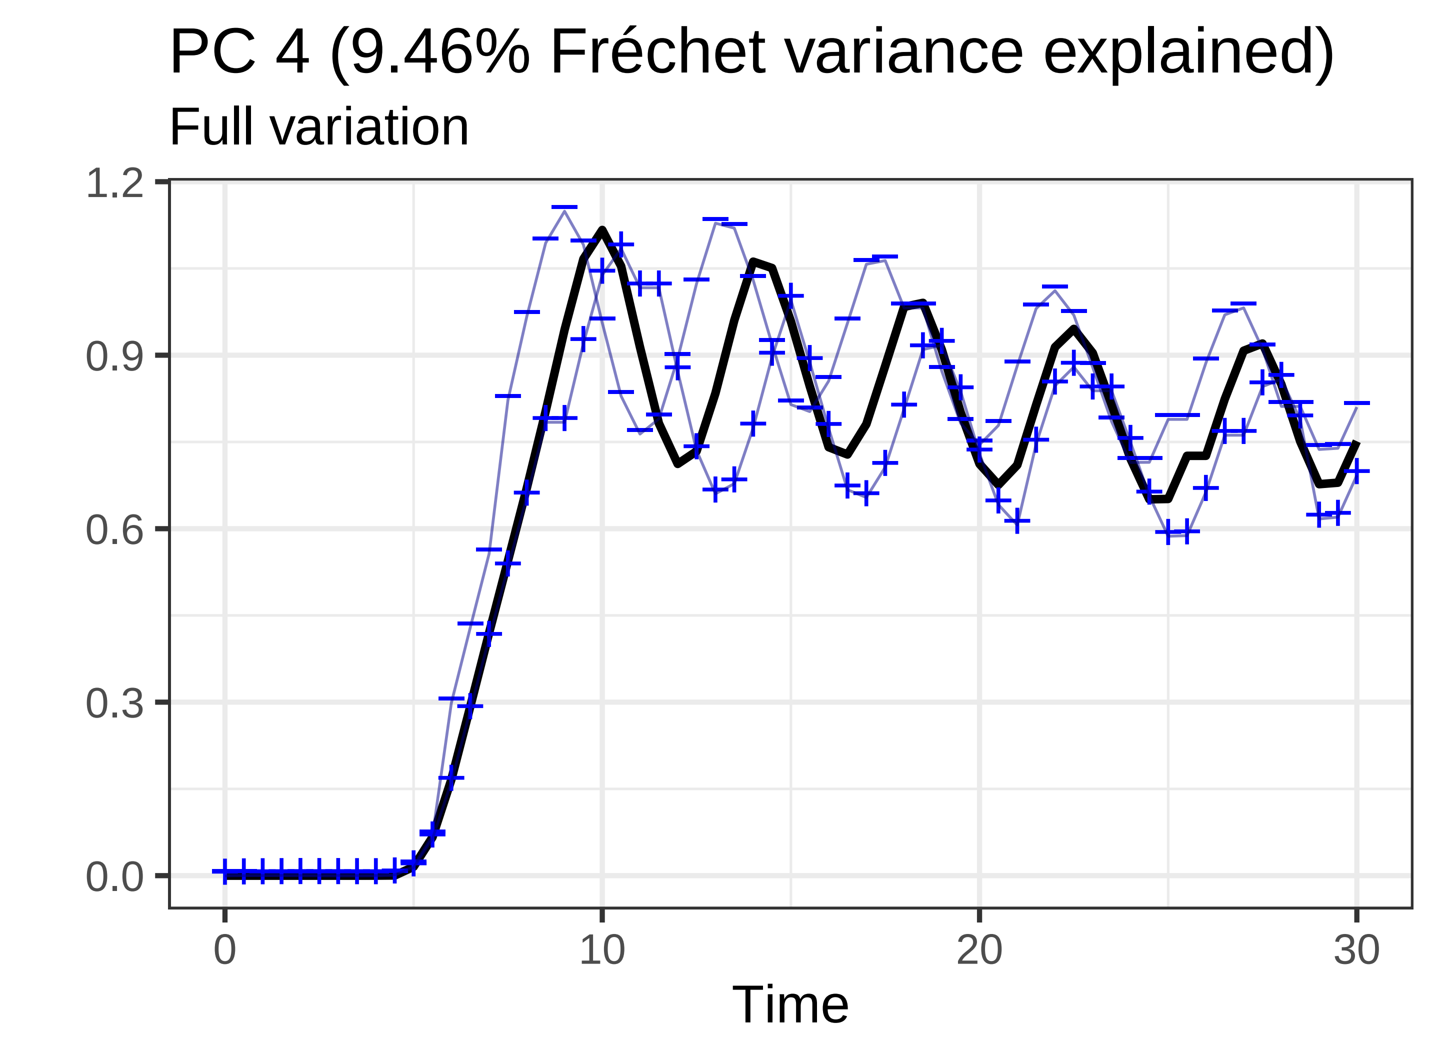
PC 4 (9.46% Fréchet variance explained)
Full variation
1.2
0.9
0.6
0.3
0.0
0
10
20
30
Time

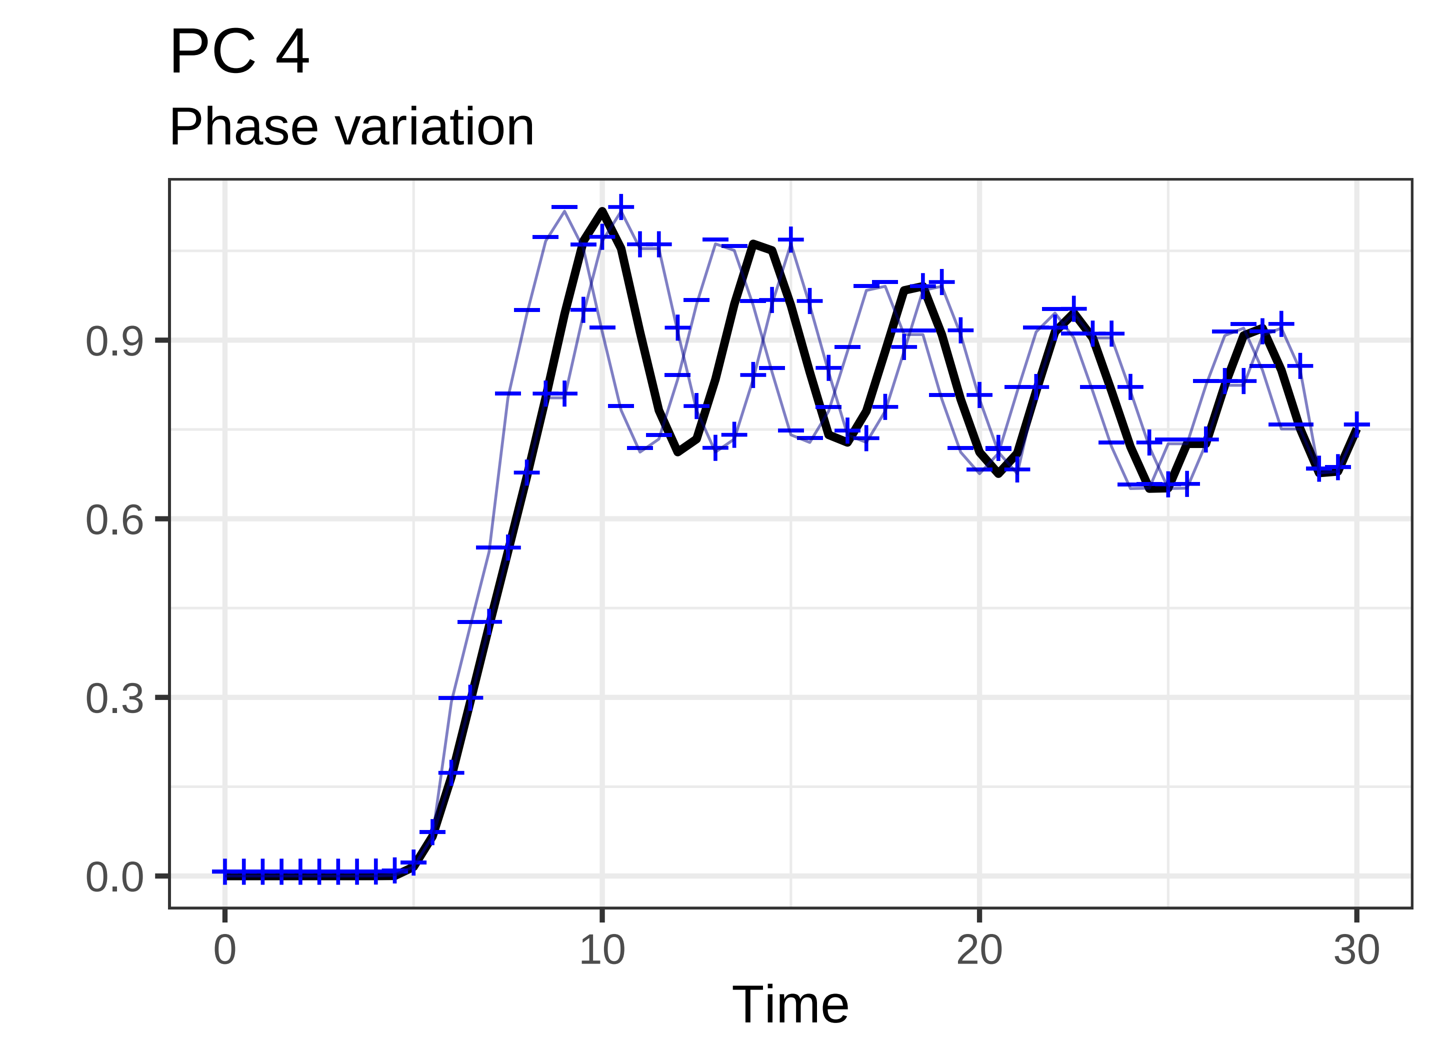

PC 4
Phase variation
0.9
0.6
0.3
0.0
0
10
20
30
Time

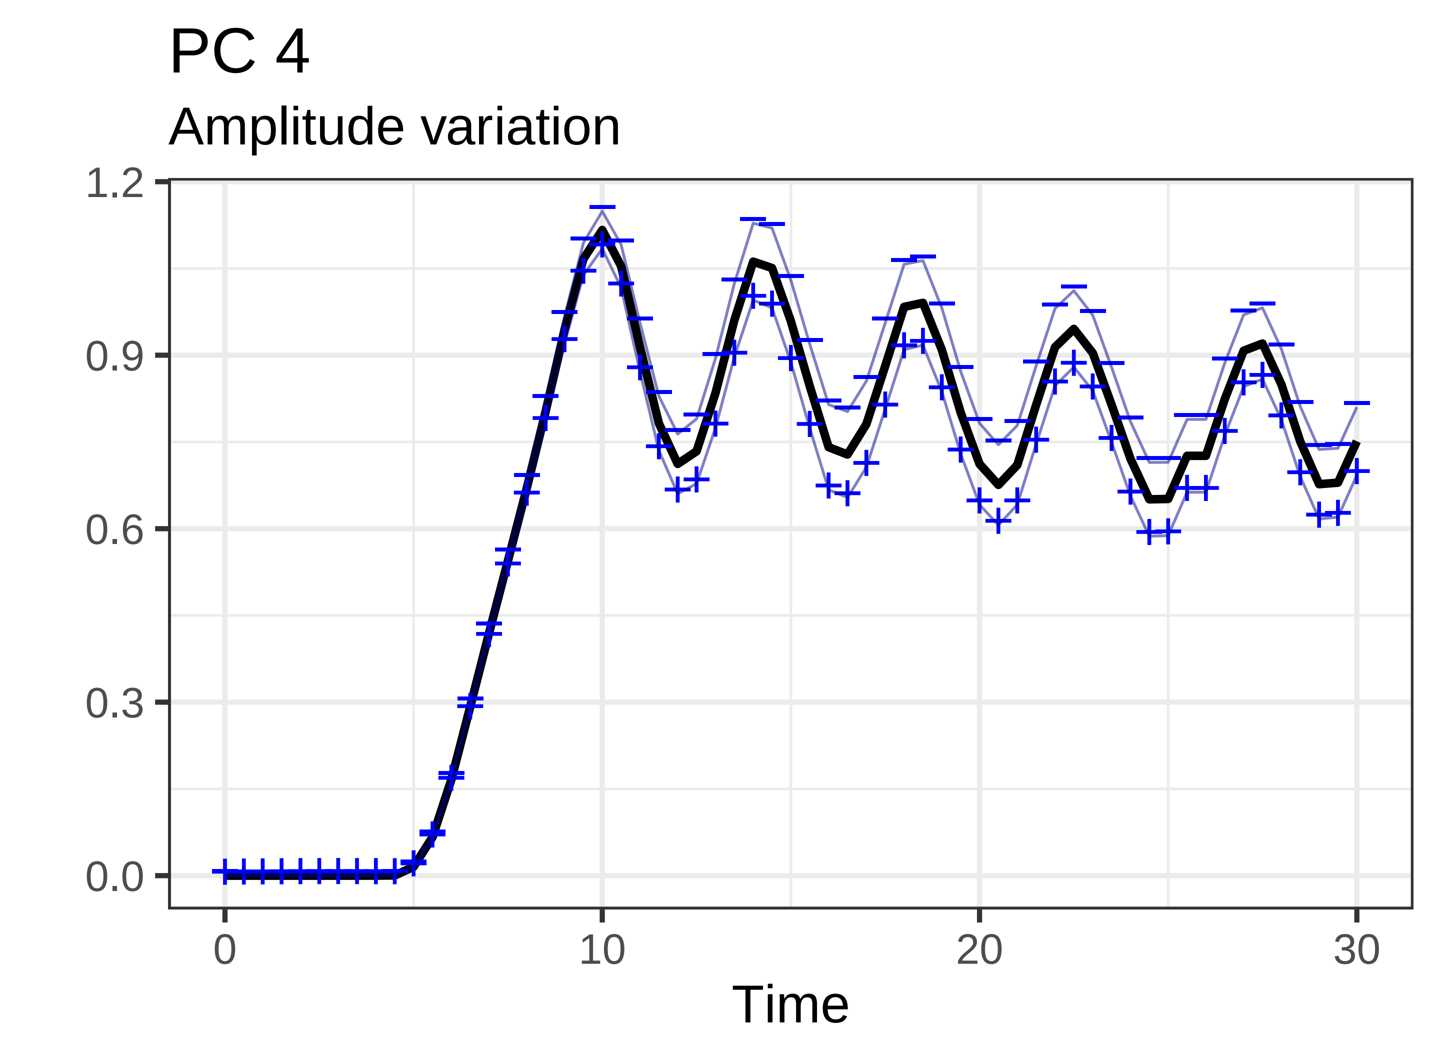
PC 4
Amplitude variation
1.2
0.9
0.6
0.3
0.0
0
10
20
30
Time

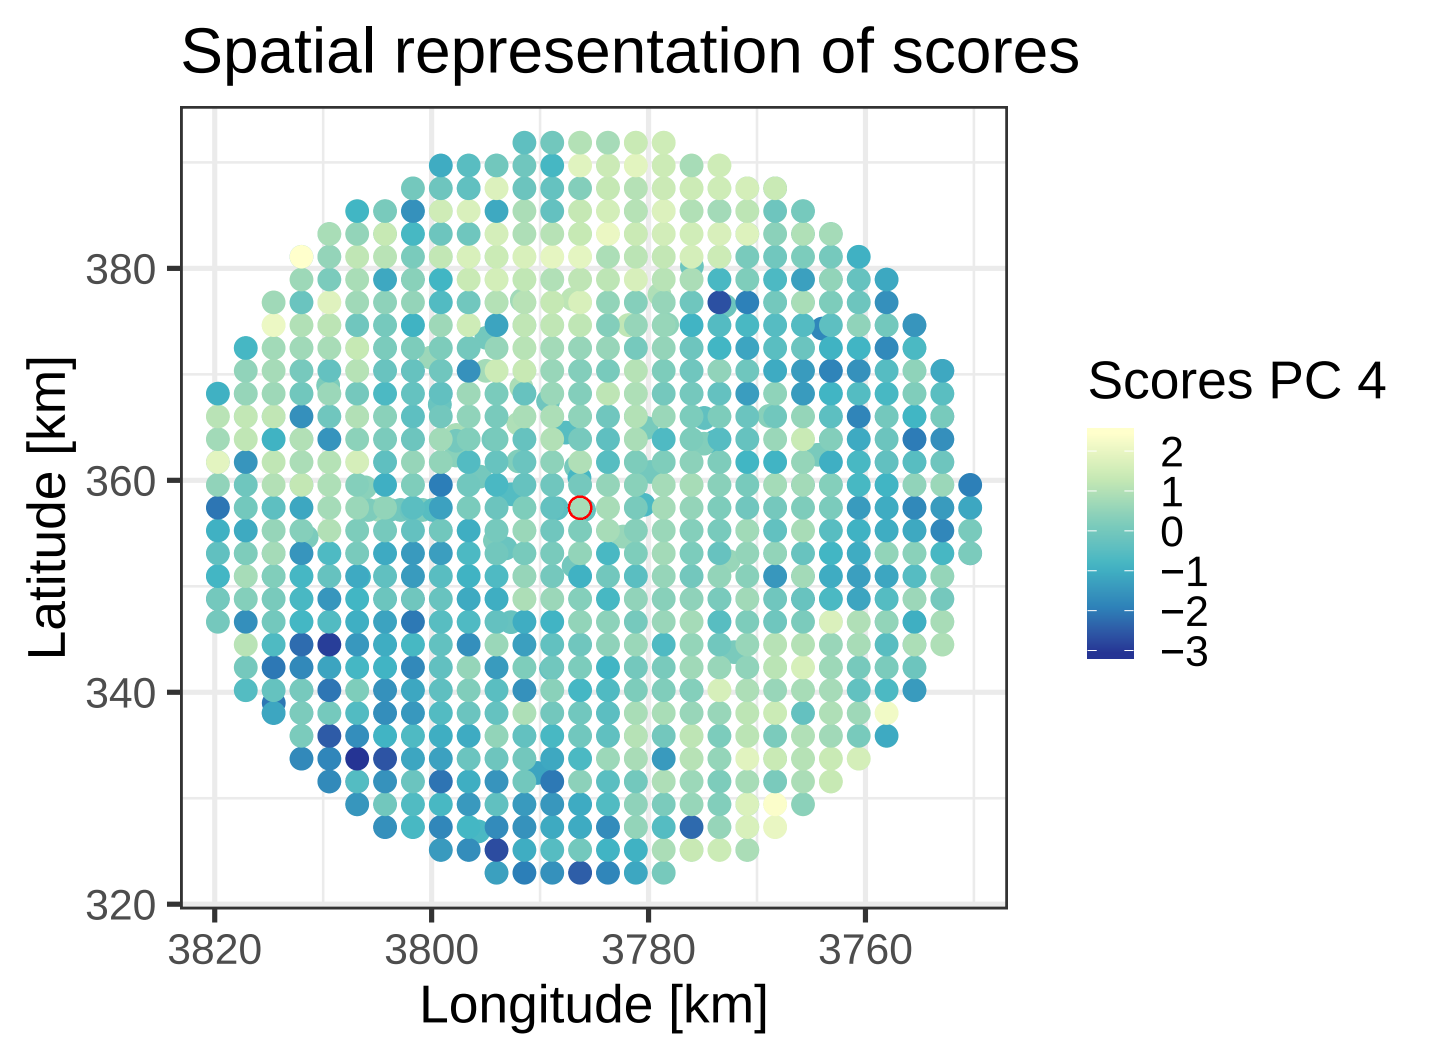

Spatial representation of scores
Latitude [km]
380
360
340
320
3820
3800
3780
3760
Longitude [km]
Scores PC 4
2
1
0
−1
−2
−3

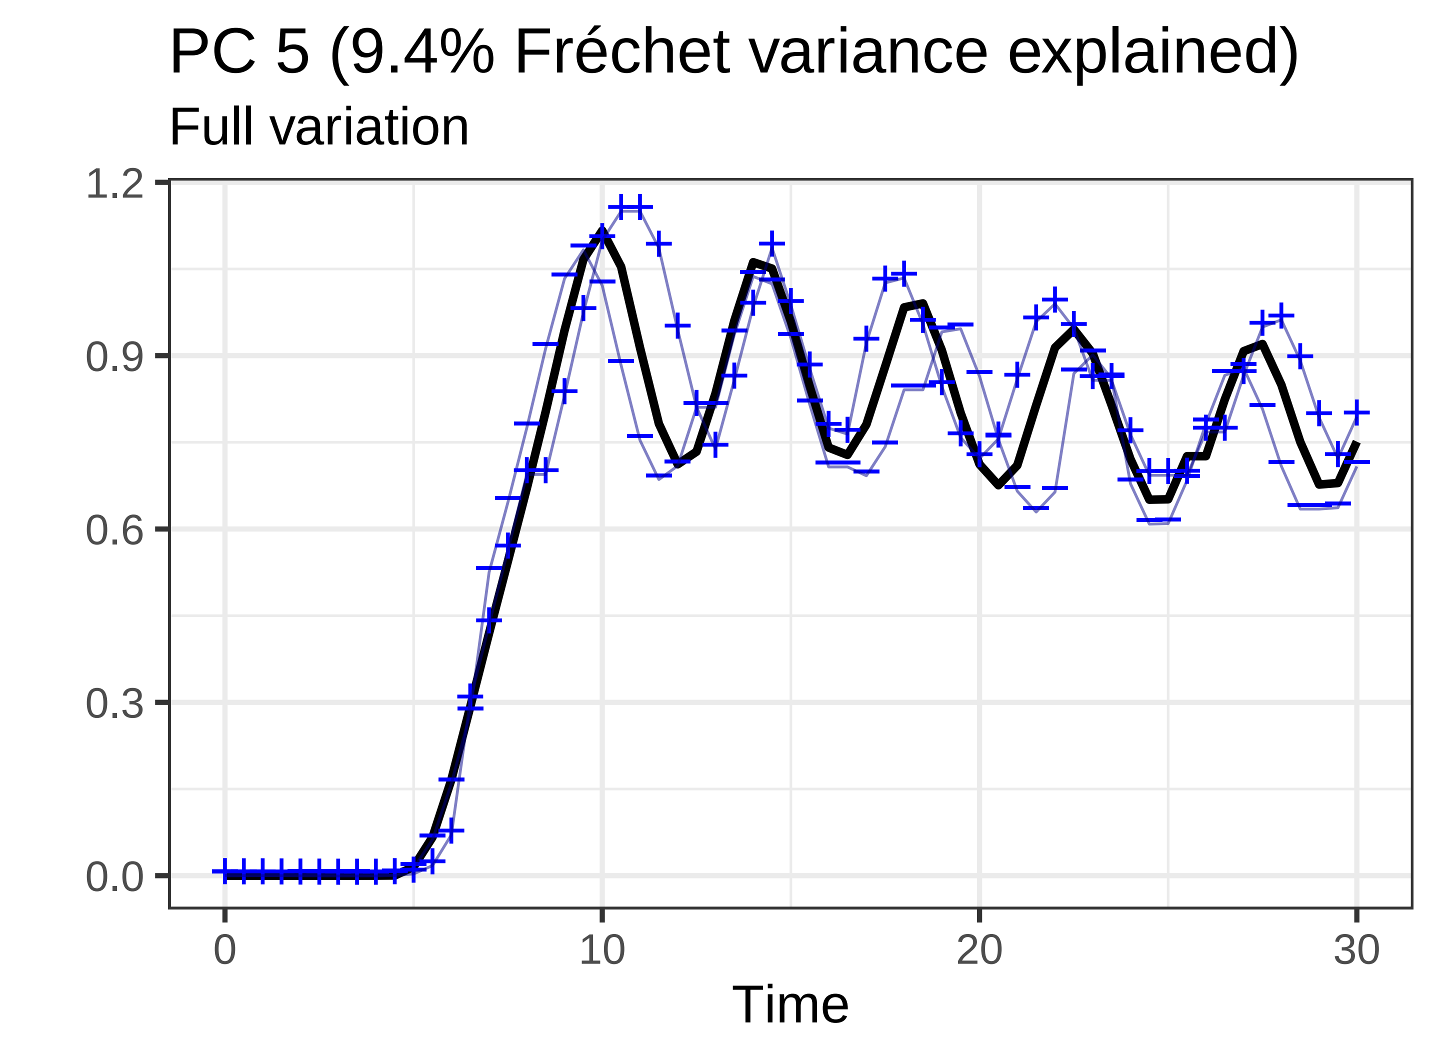

PC 5 (9.4% Fréchet variance explained)
Full variation
1.2
0.9
0.6
0.3
0.0
0
10
20
30
Time

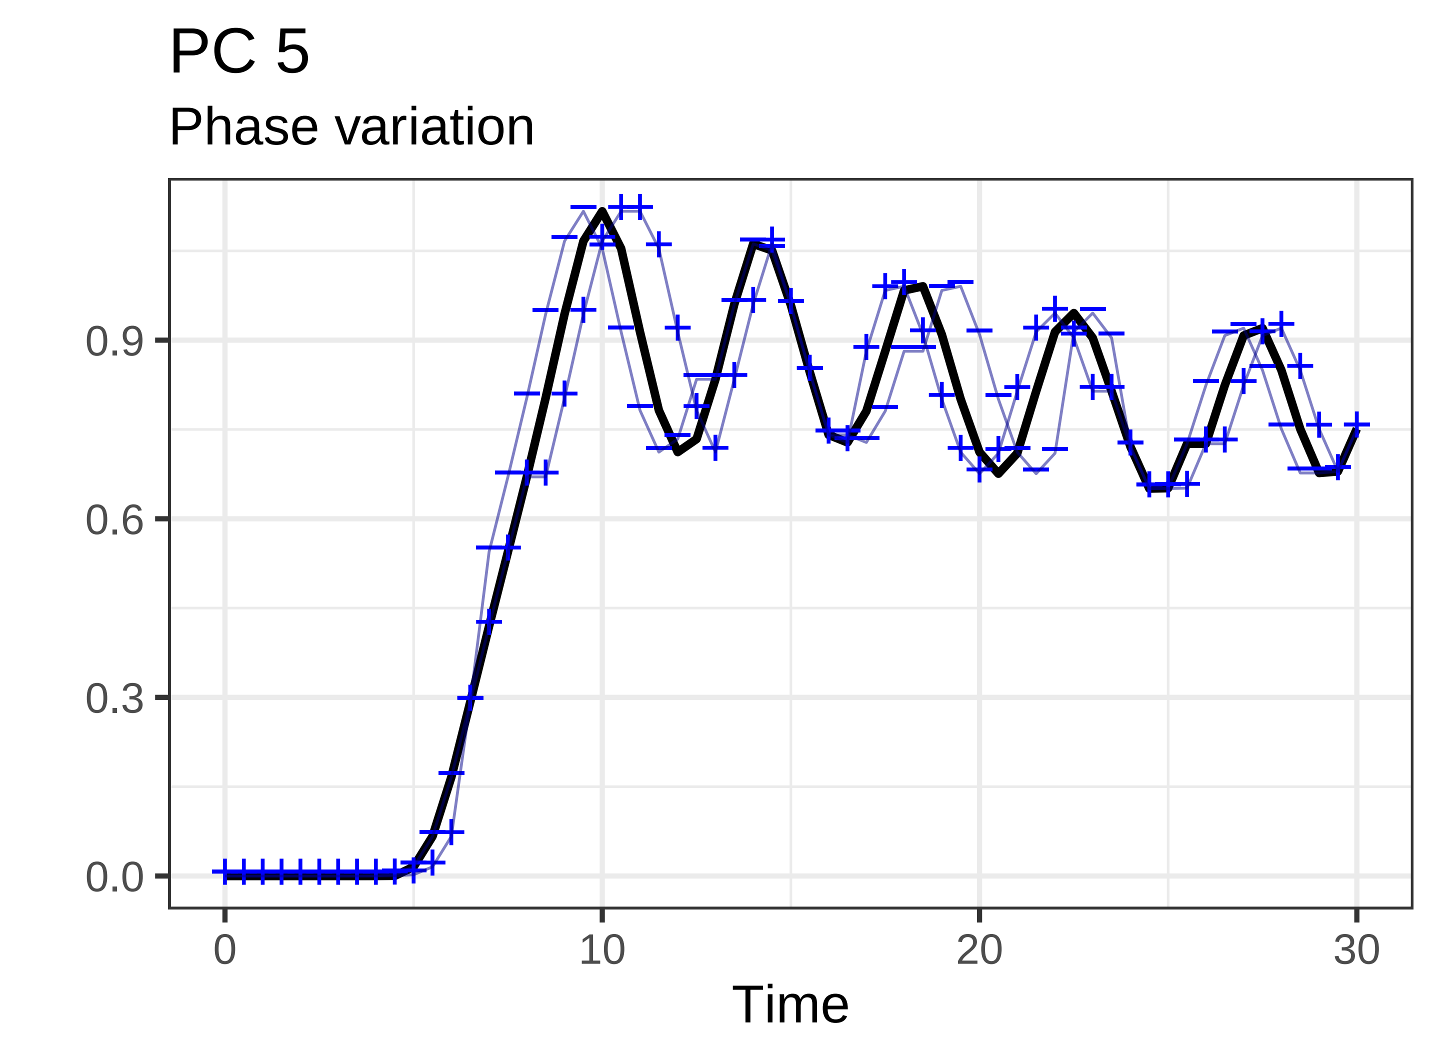
PC 5
Phase variation
0.9
0.6
0.3
0.0
0
10
20
30
Time

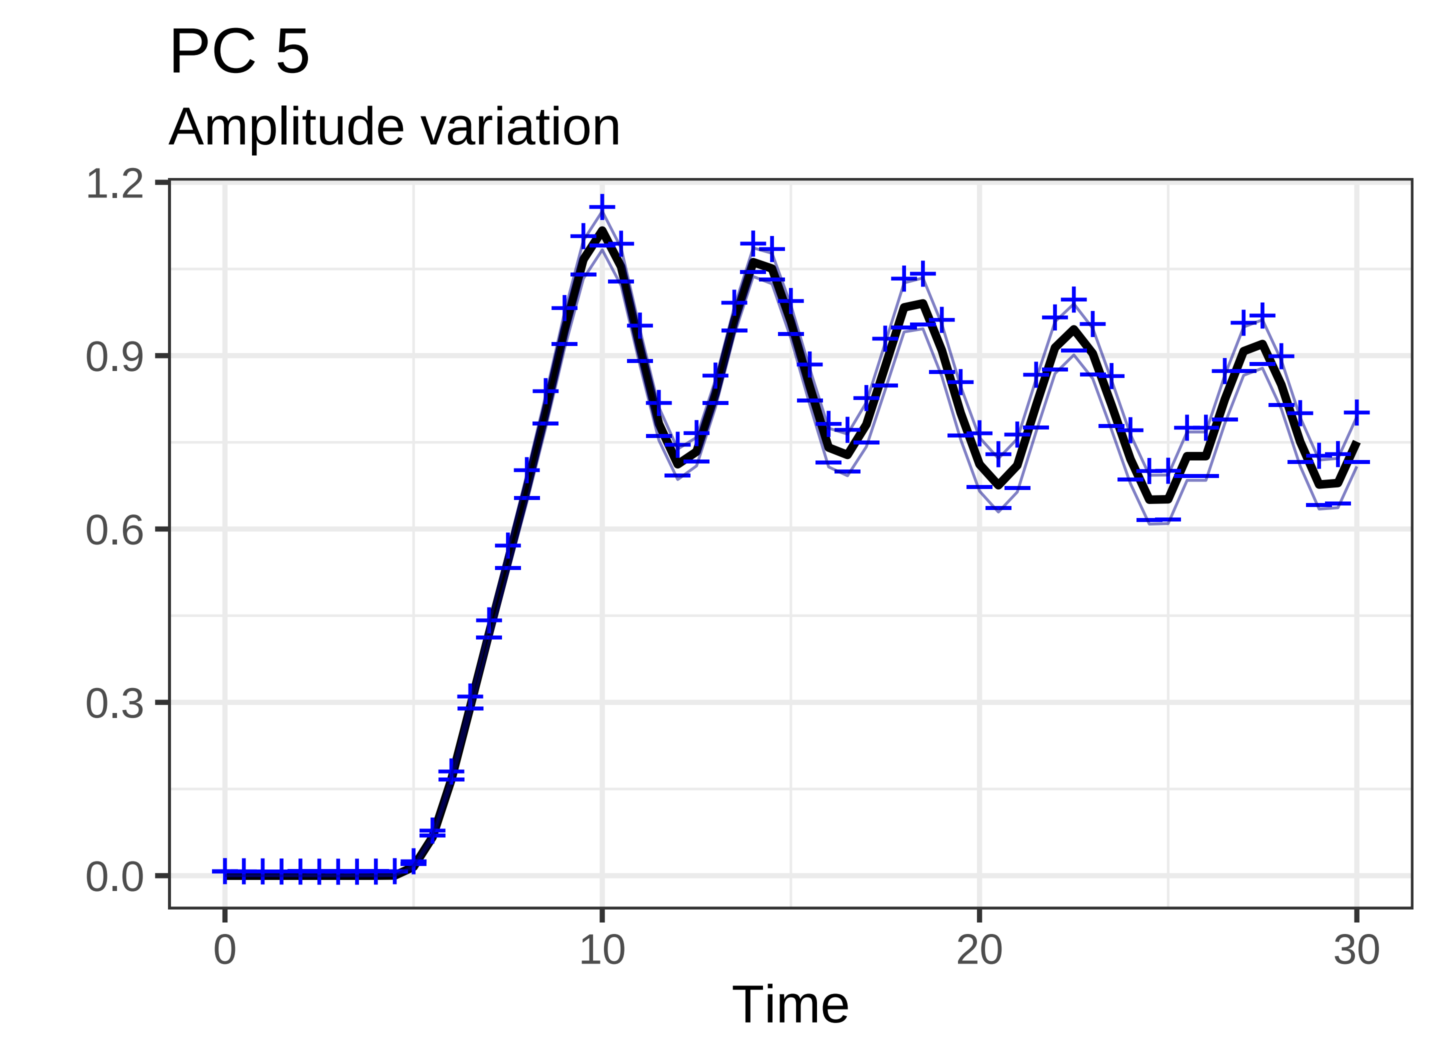

PC 5
Amplitude variation
1.2
0.9
0.6
0.3
0.0
0
10
20
30
Time

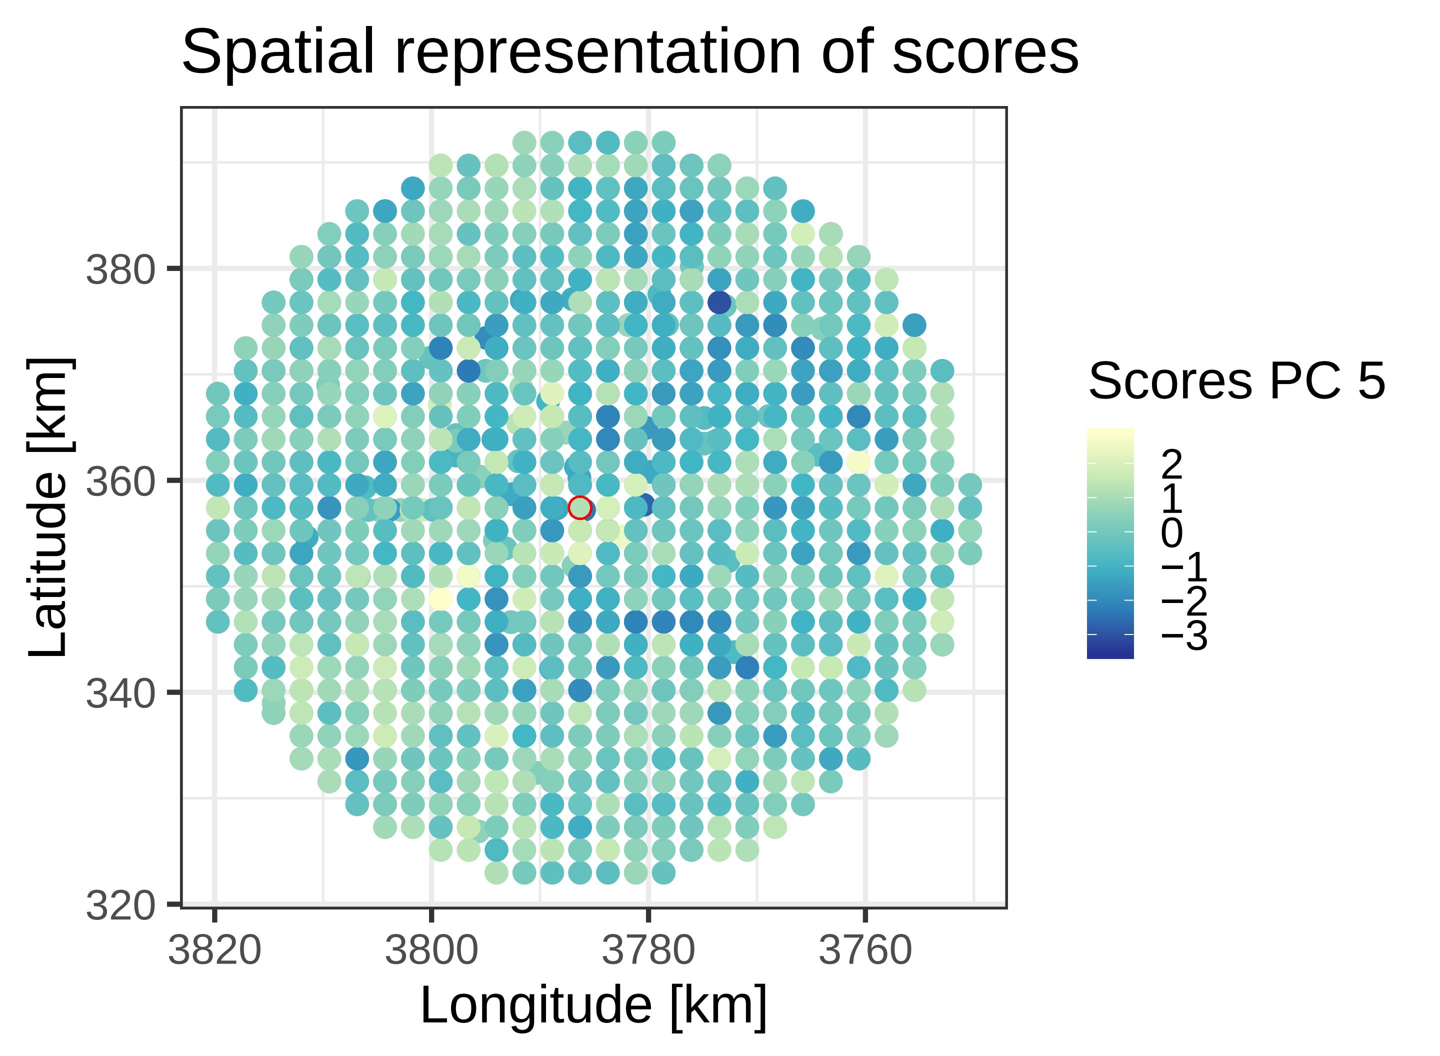
Spatial representation of scores
Latitude [km]
380
360
340
320
Longitude [km]
3820
3800
3780
3760
Scores PC 5
2
1
0
−1
−2
−3

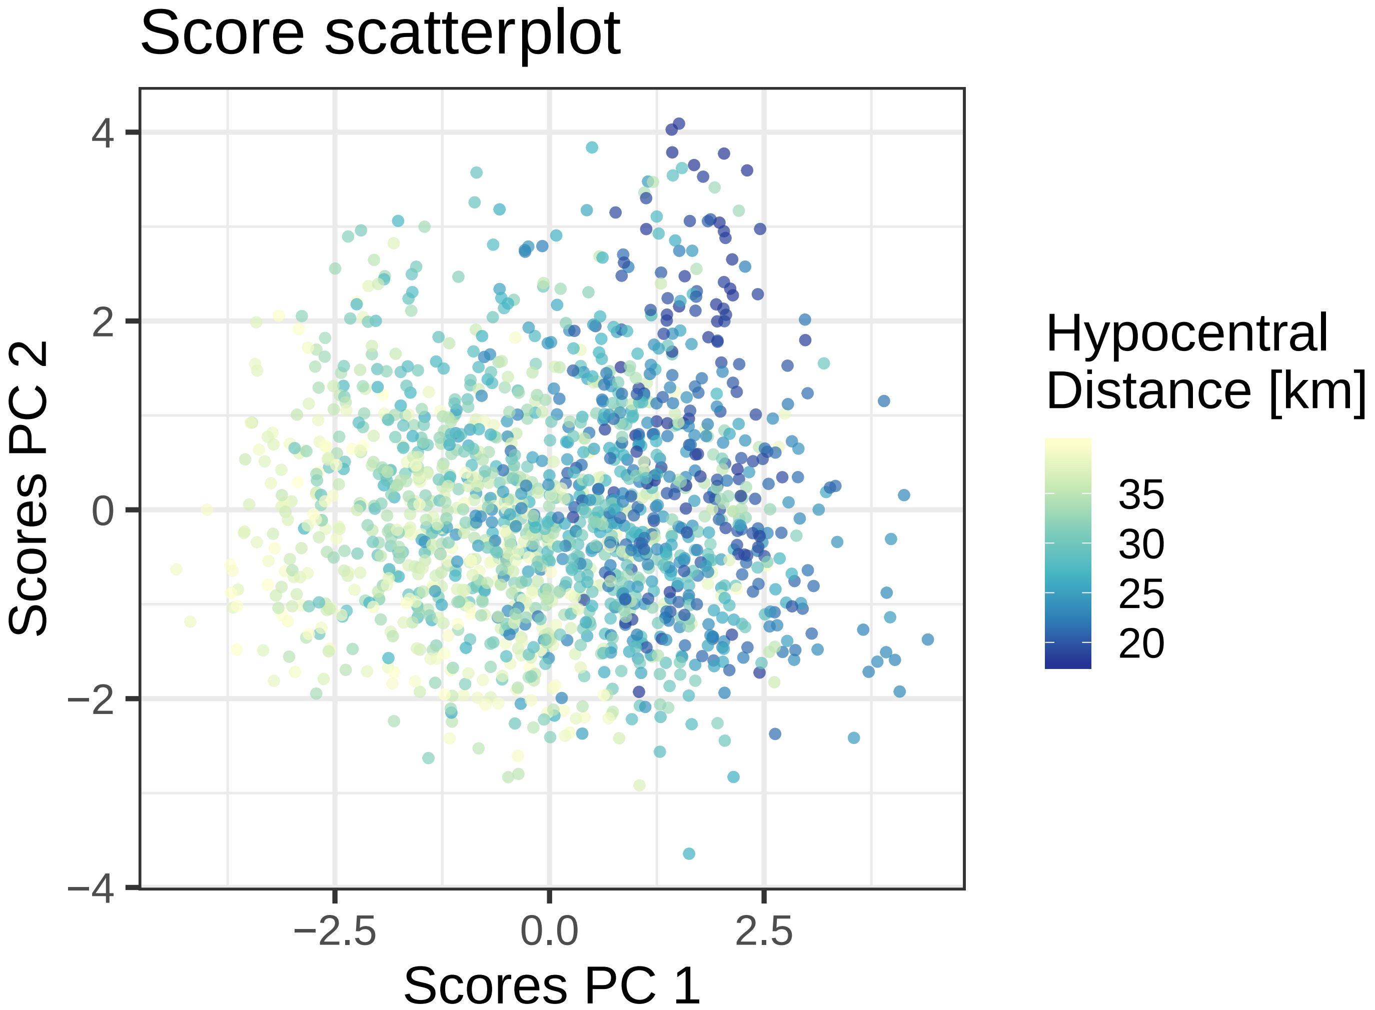

Score scatterplot
Scores PC 2
4
2
0
−2
−4
−2.5
0.0
2.5
Scores PC 1
Hypocentral
Distance [km]
35
30
25
20
