# Supplementary material for: A General Framework for Multivariate Functional Principal Component Analysis of Amplitude and Phase Variation
Source: arXiv:1810.13321 source file (2018-10-31)

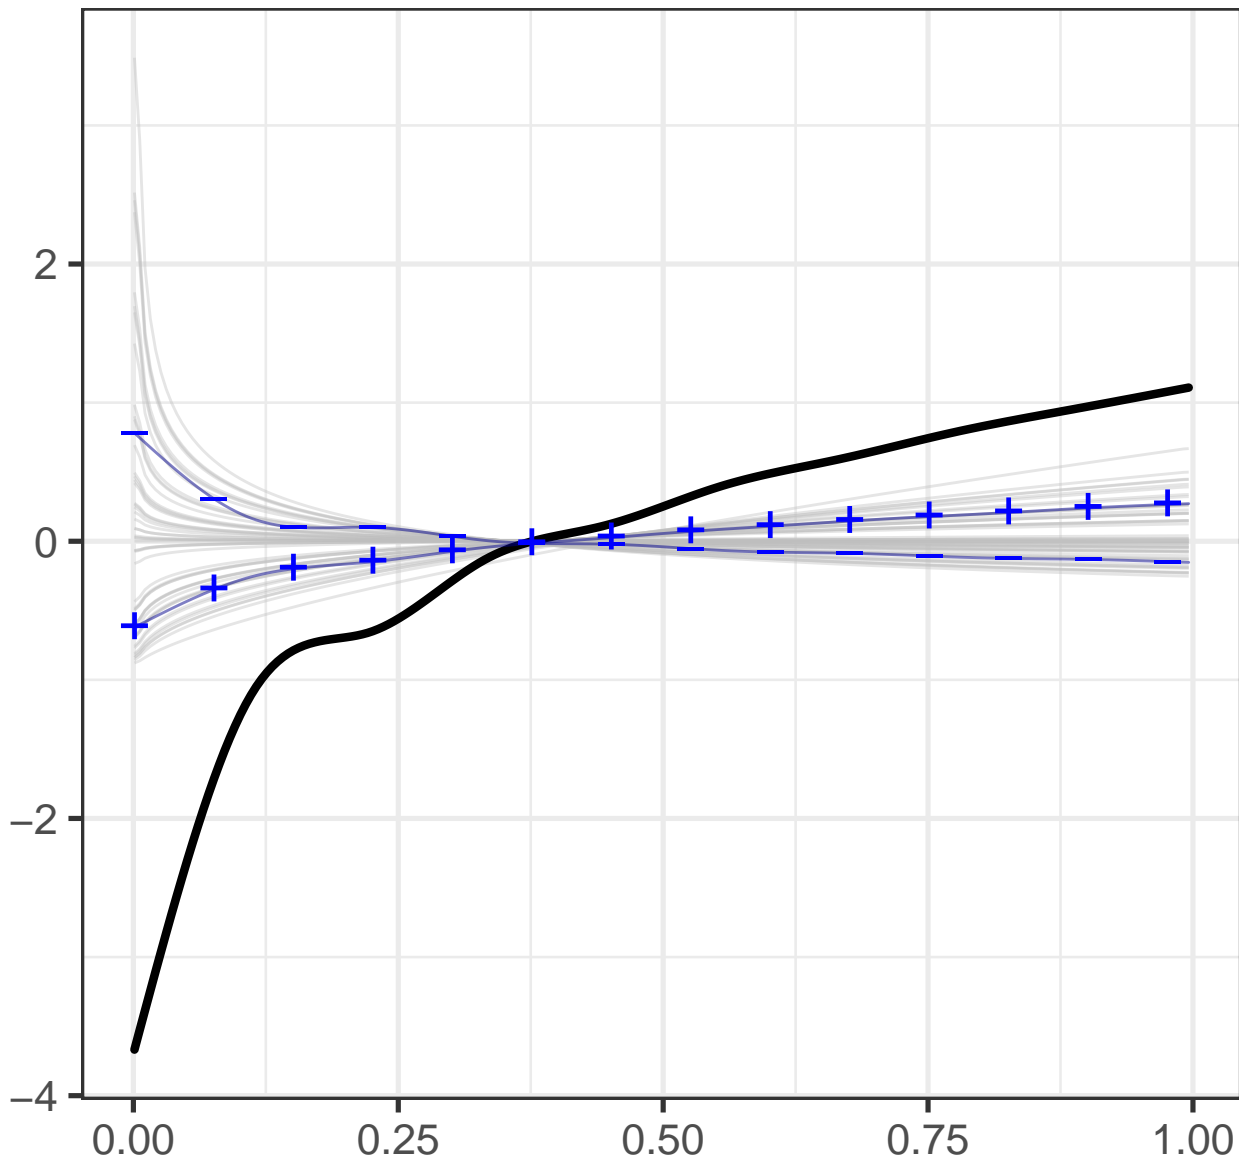

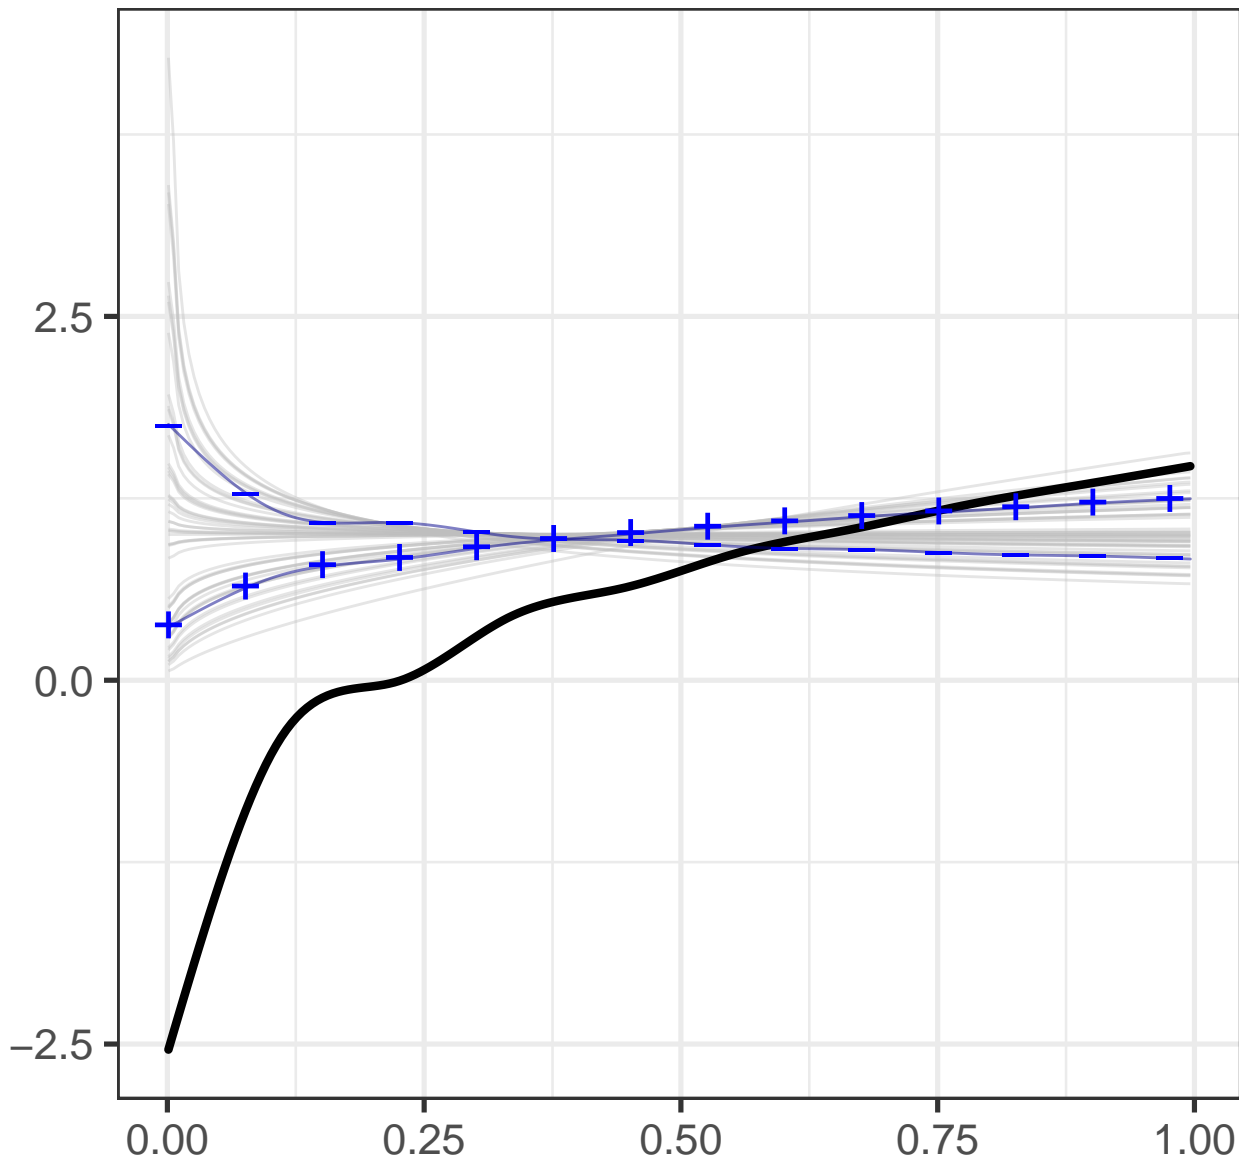

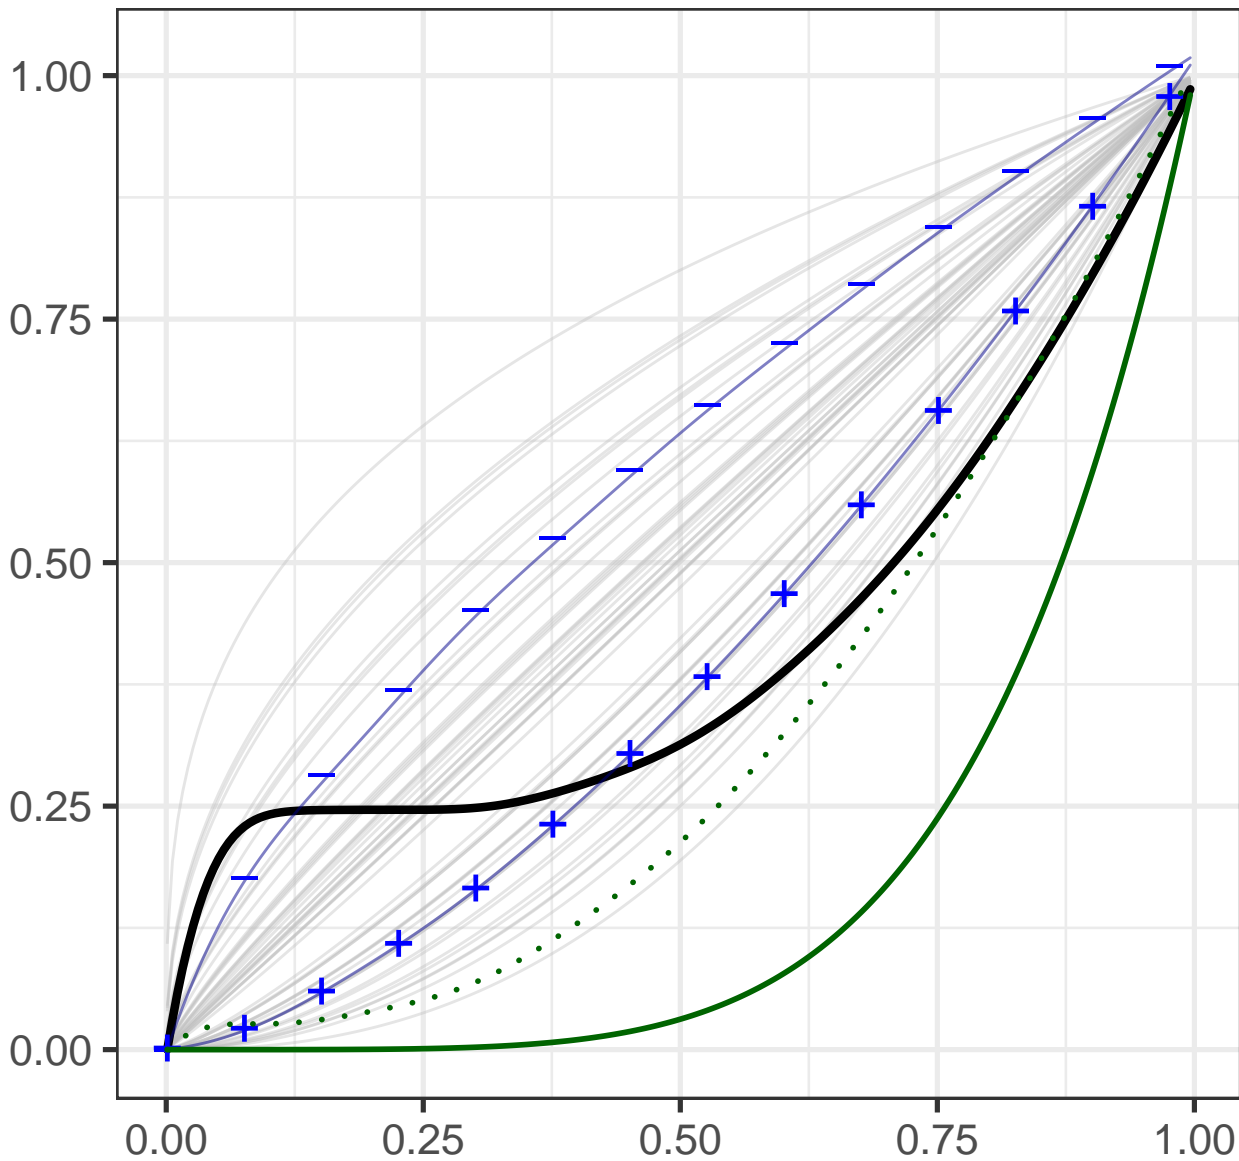

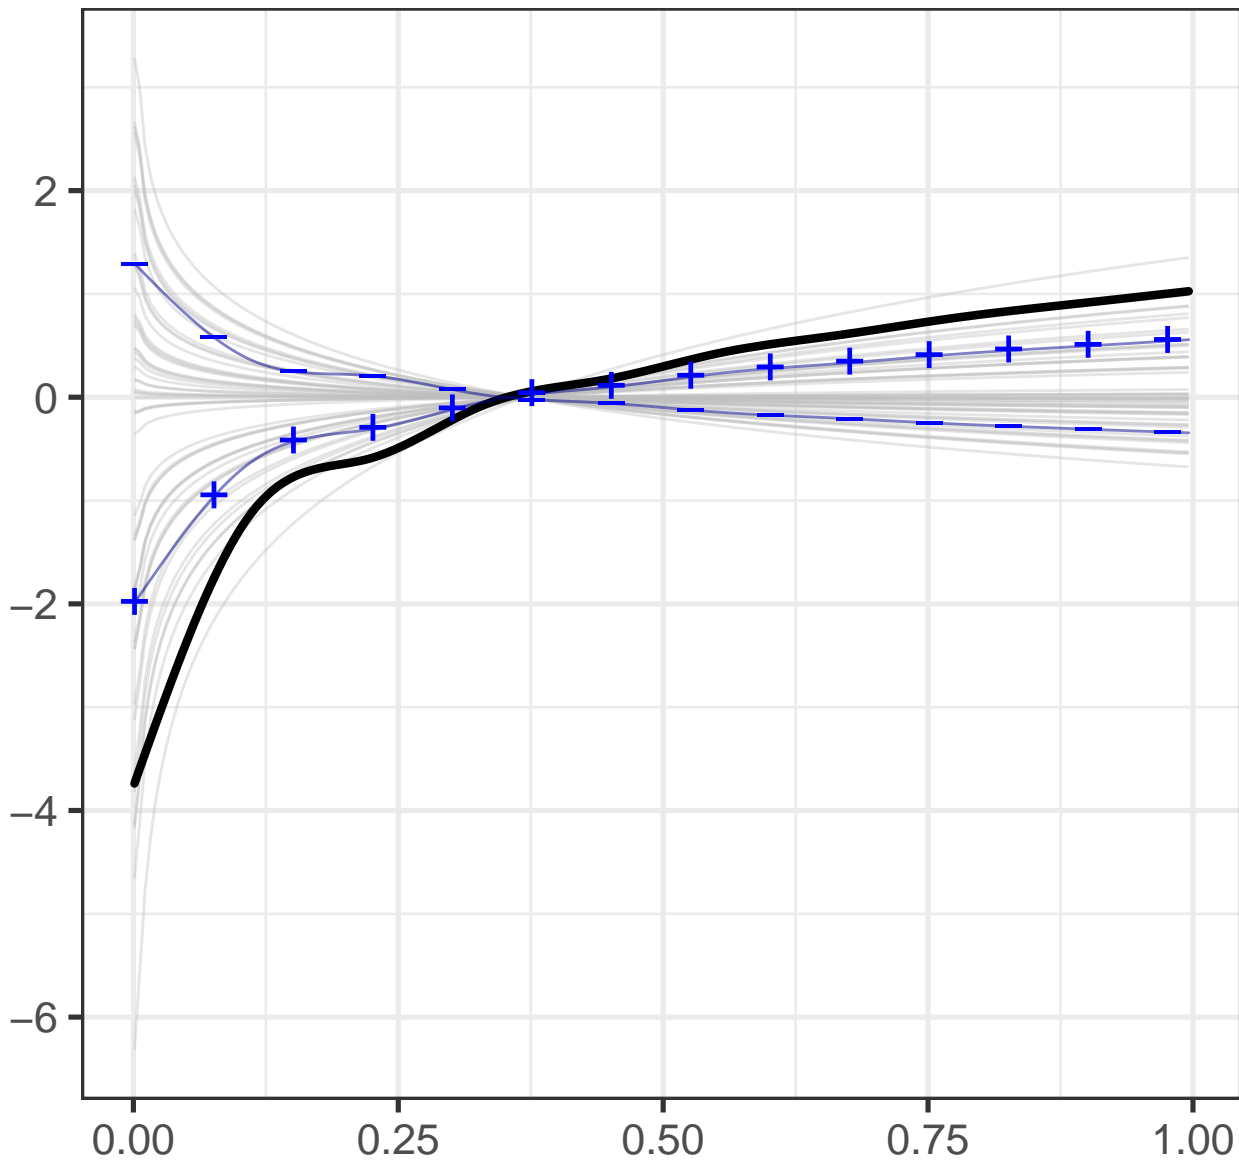

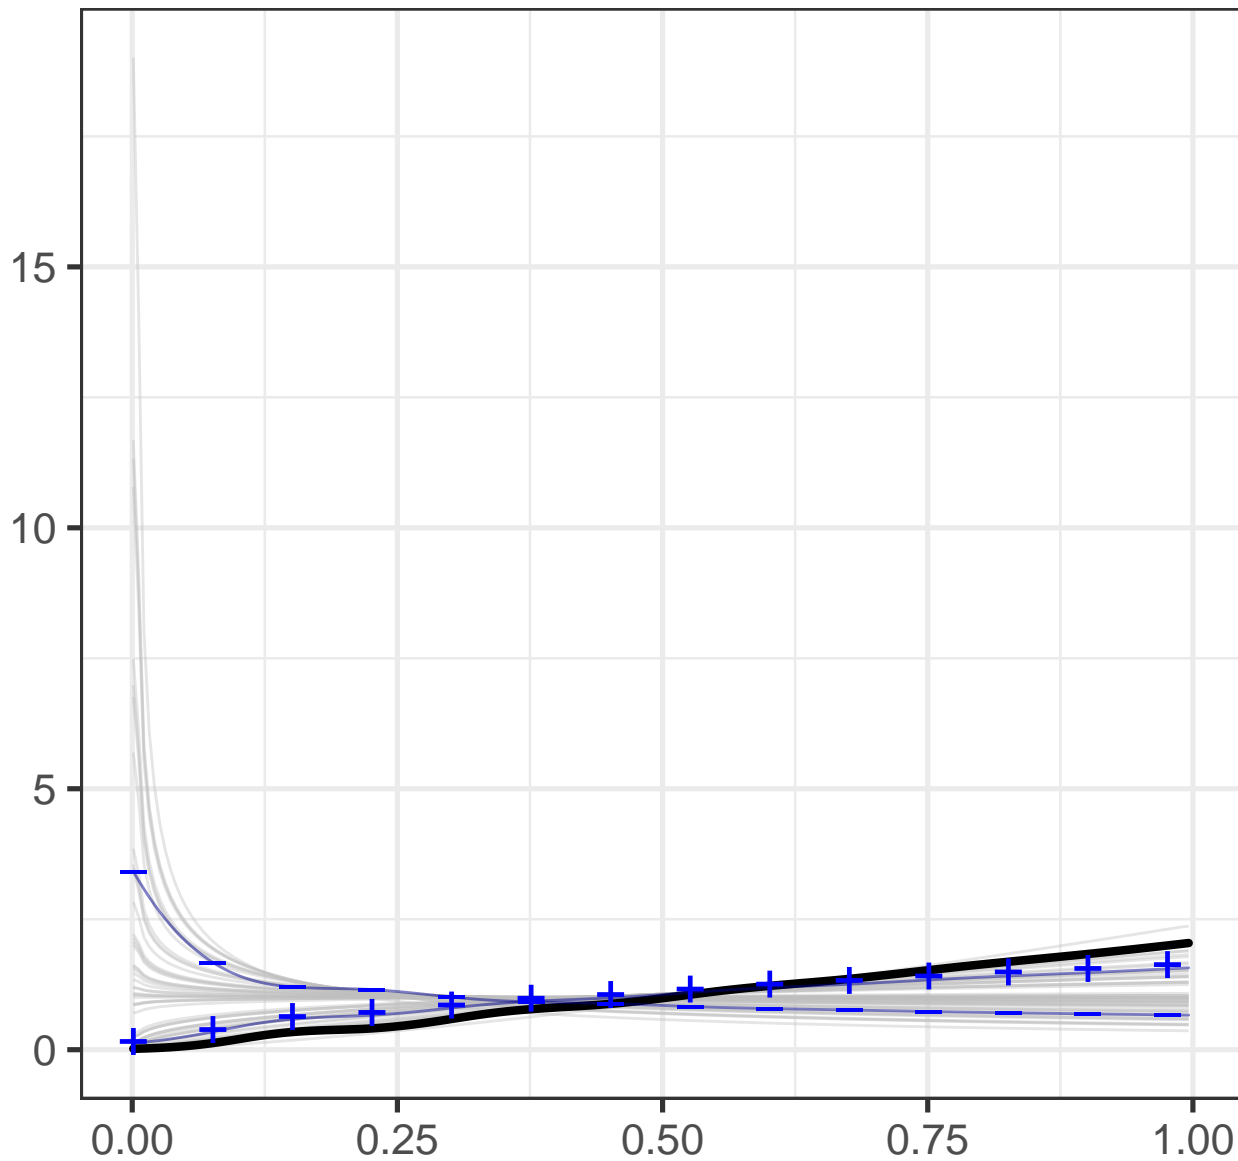

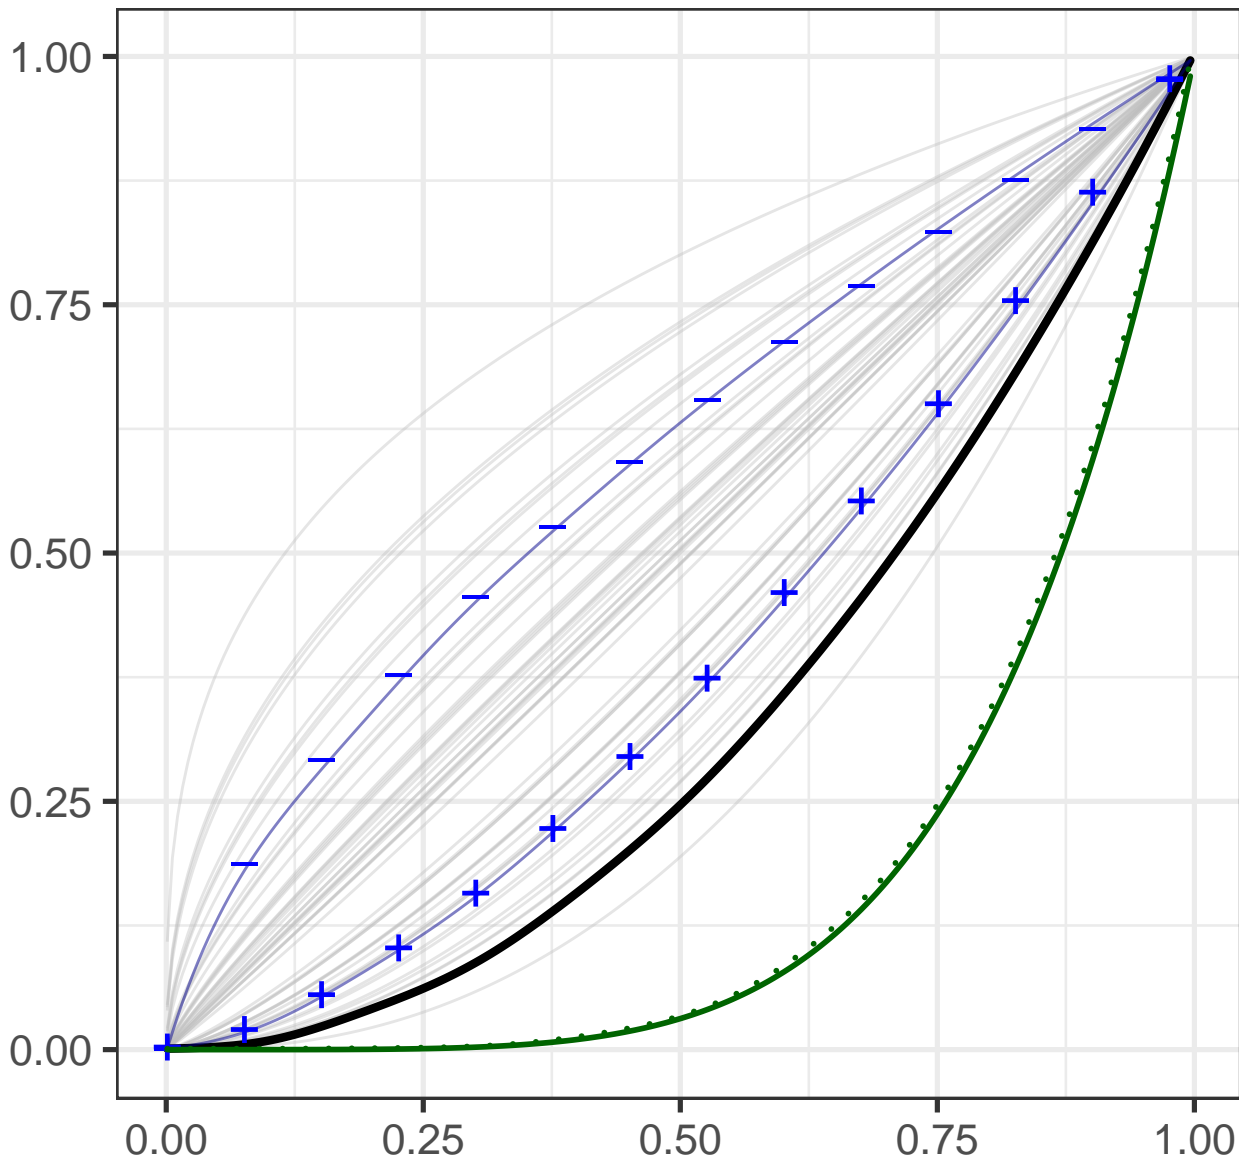

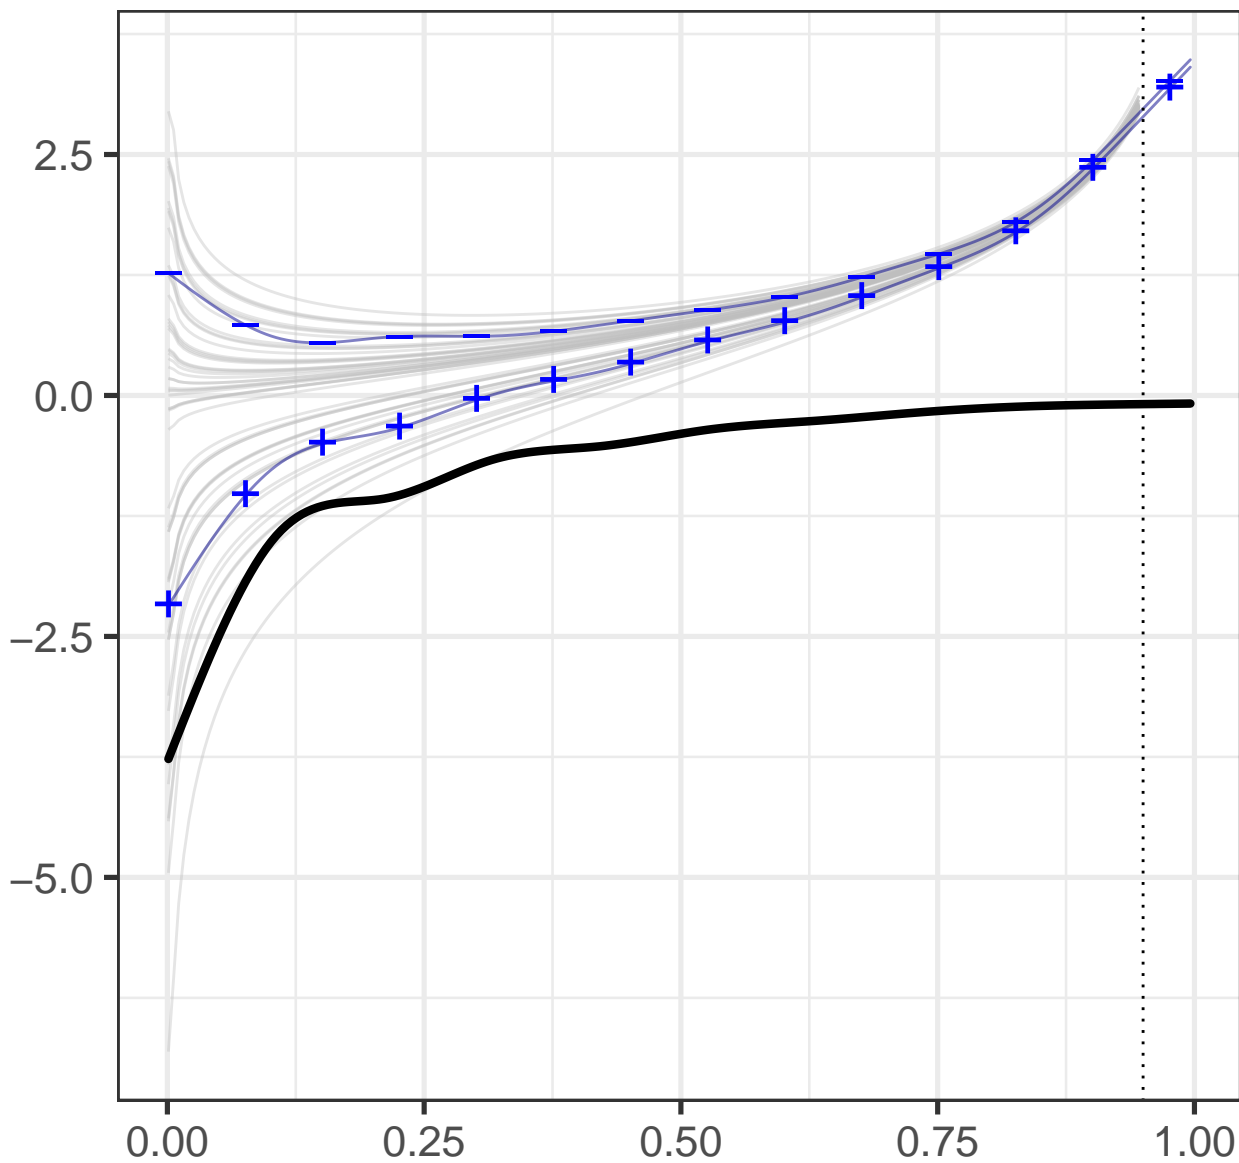

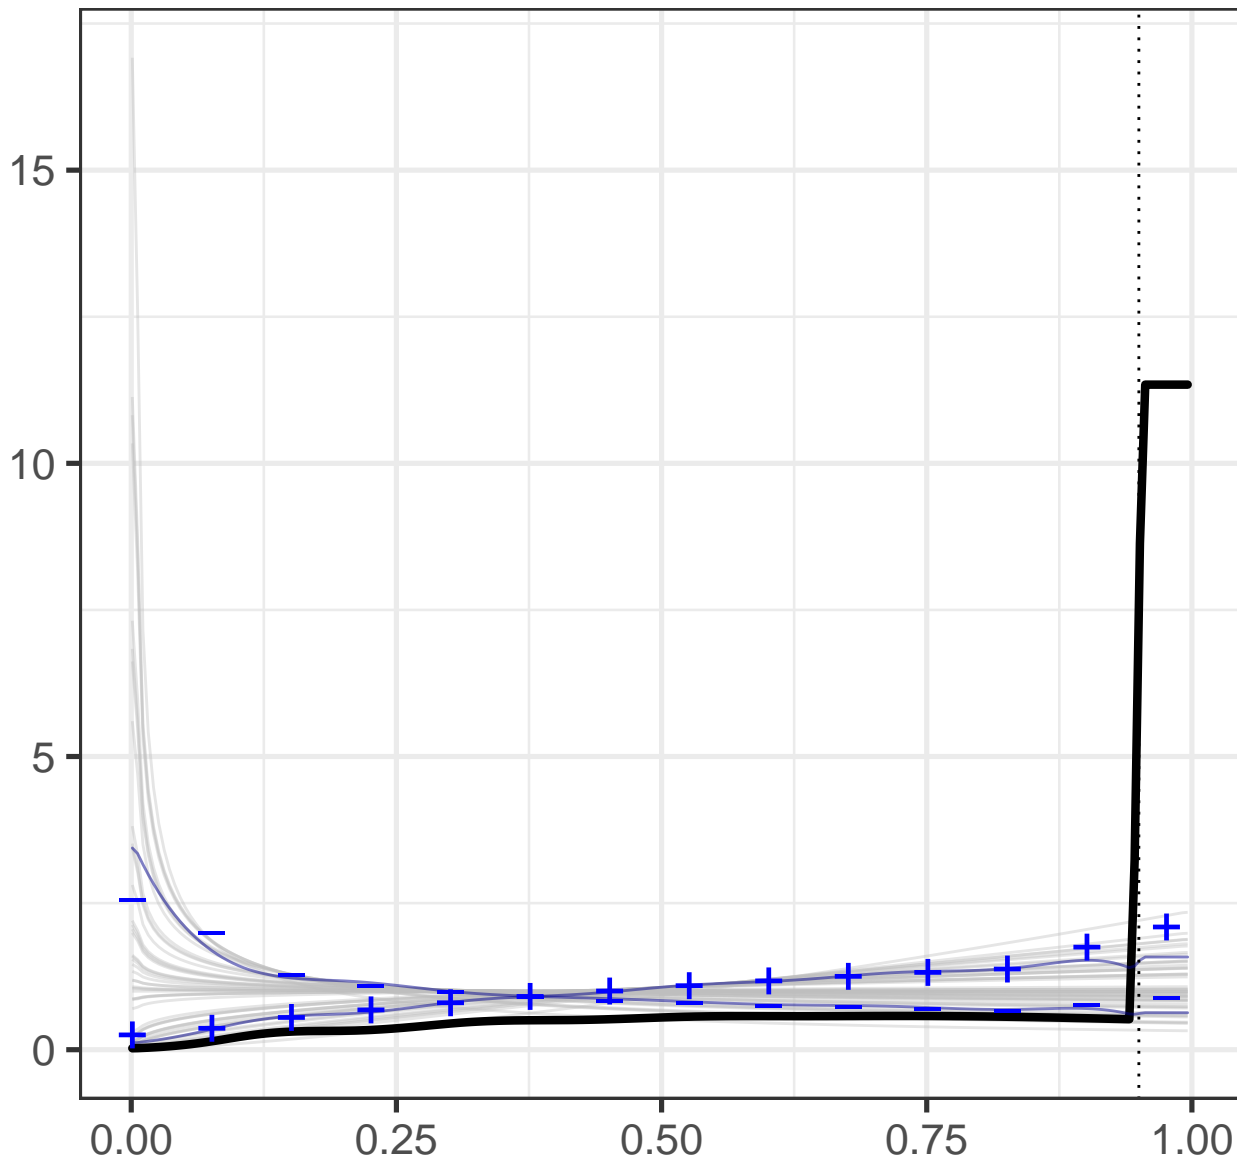



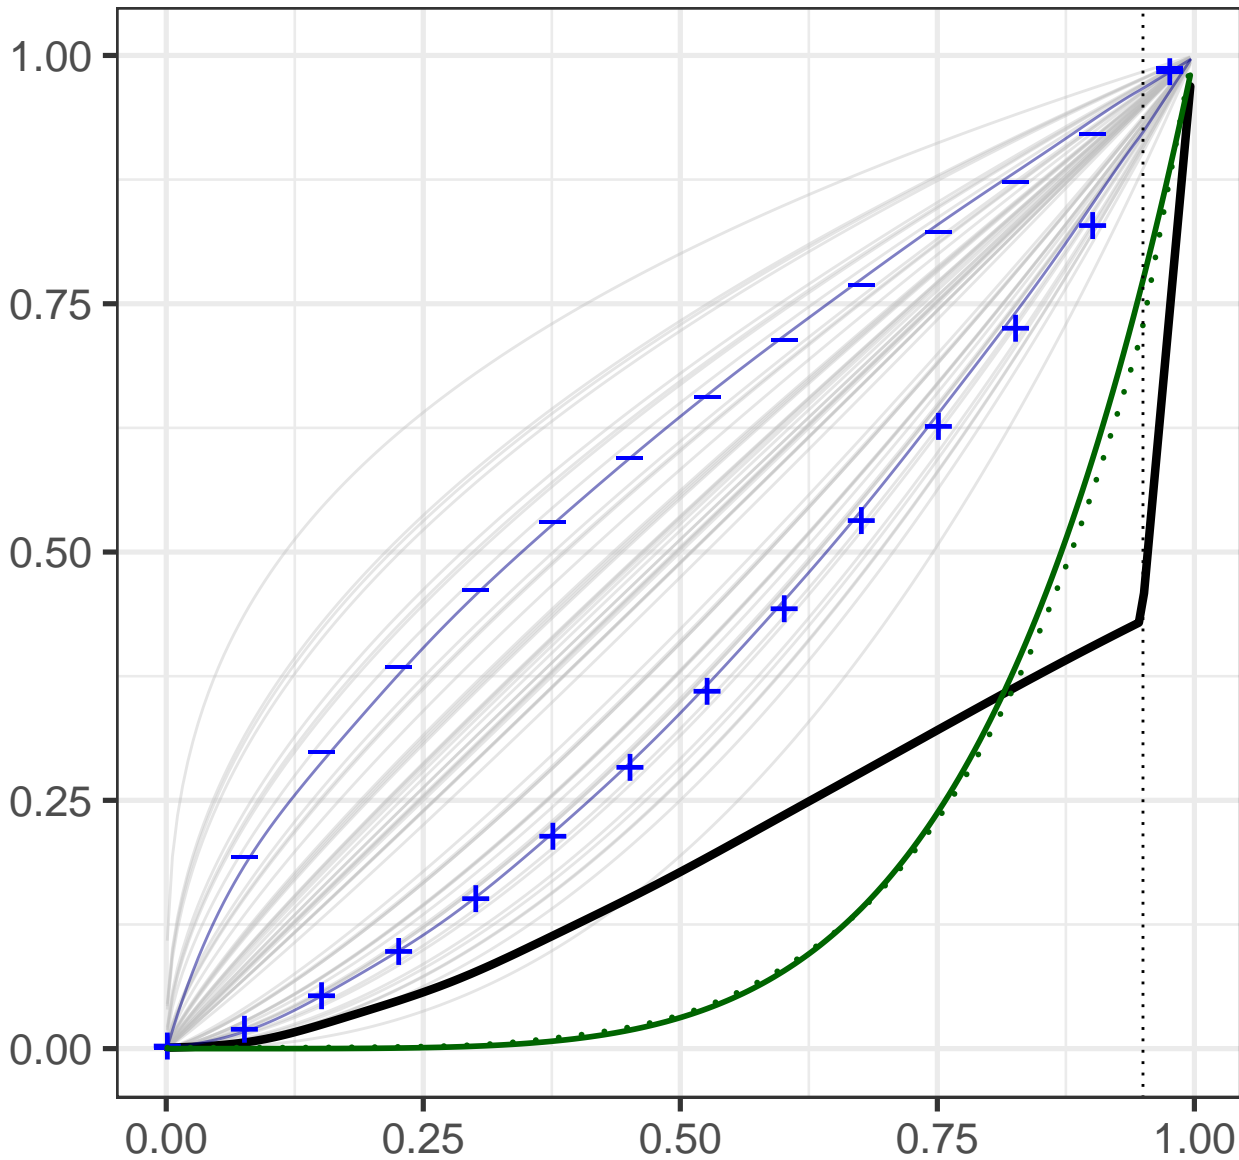

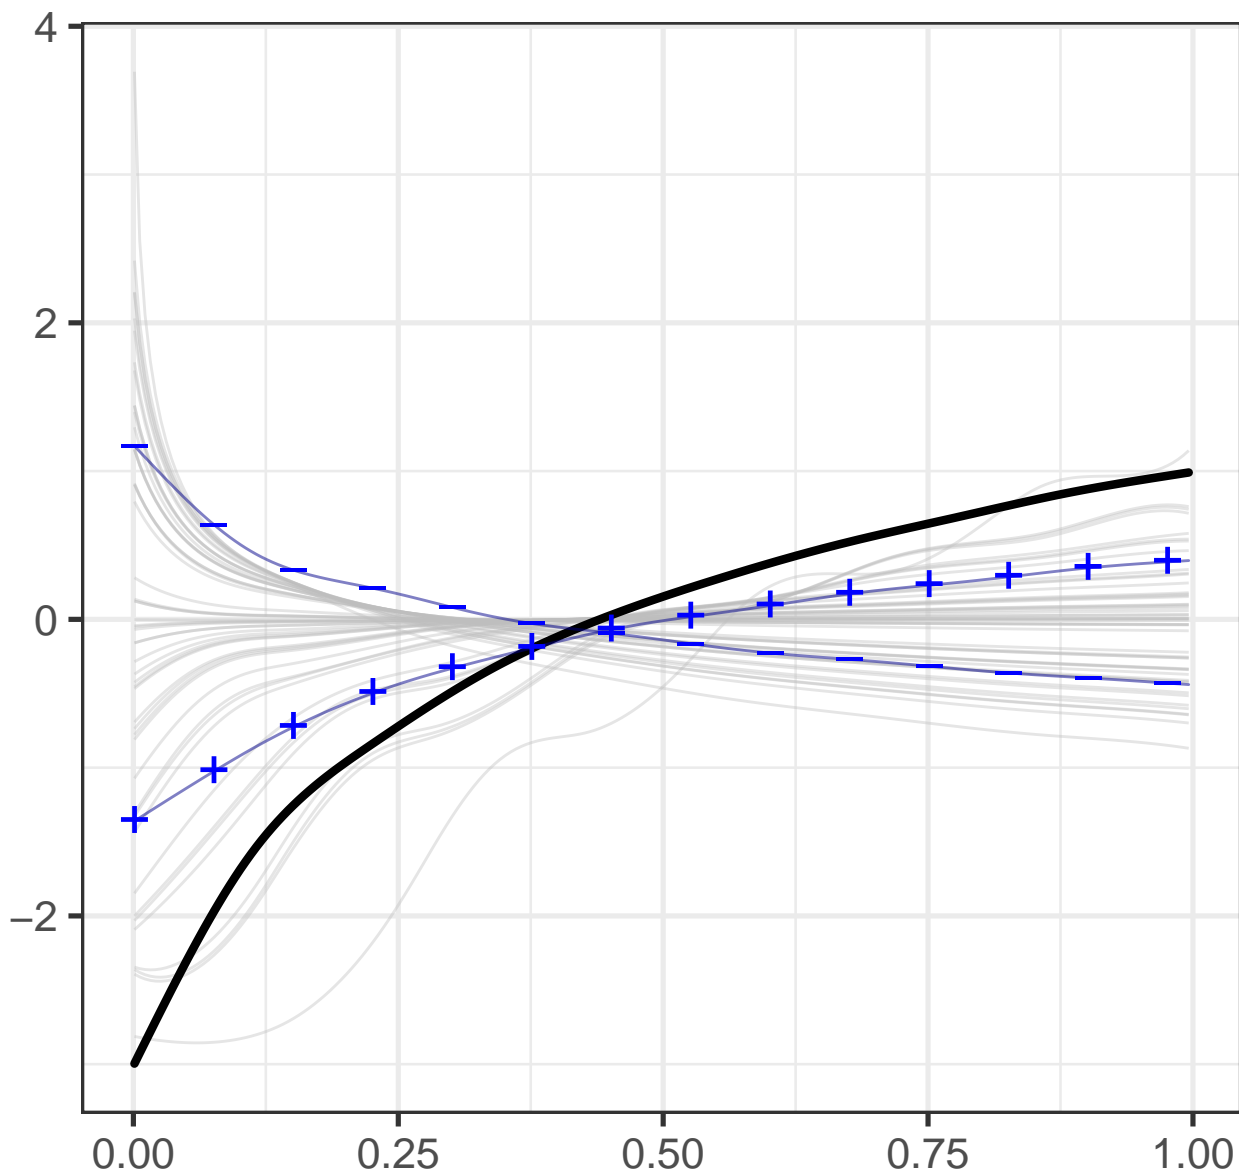

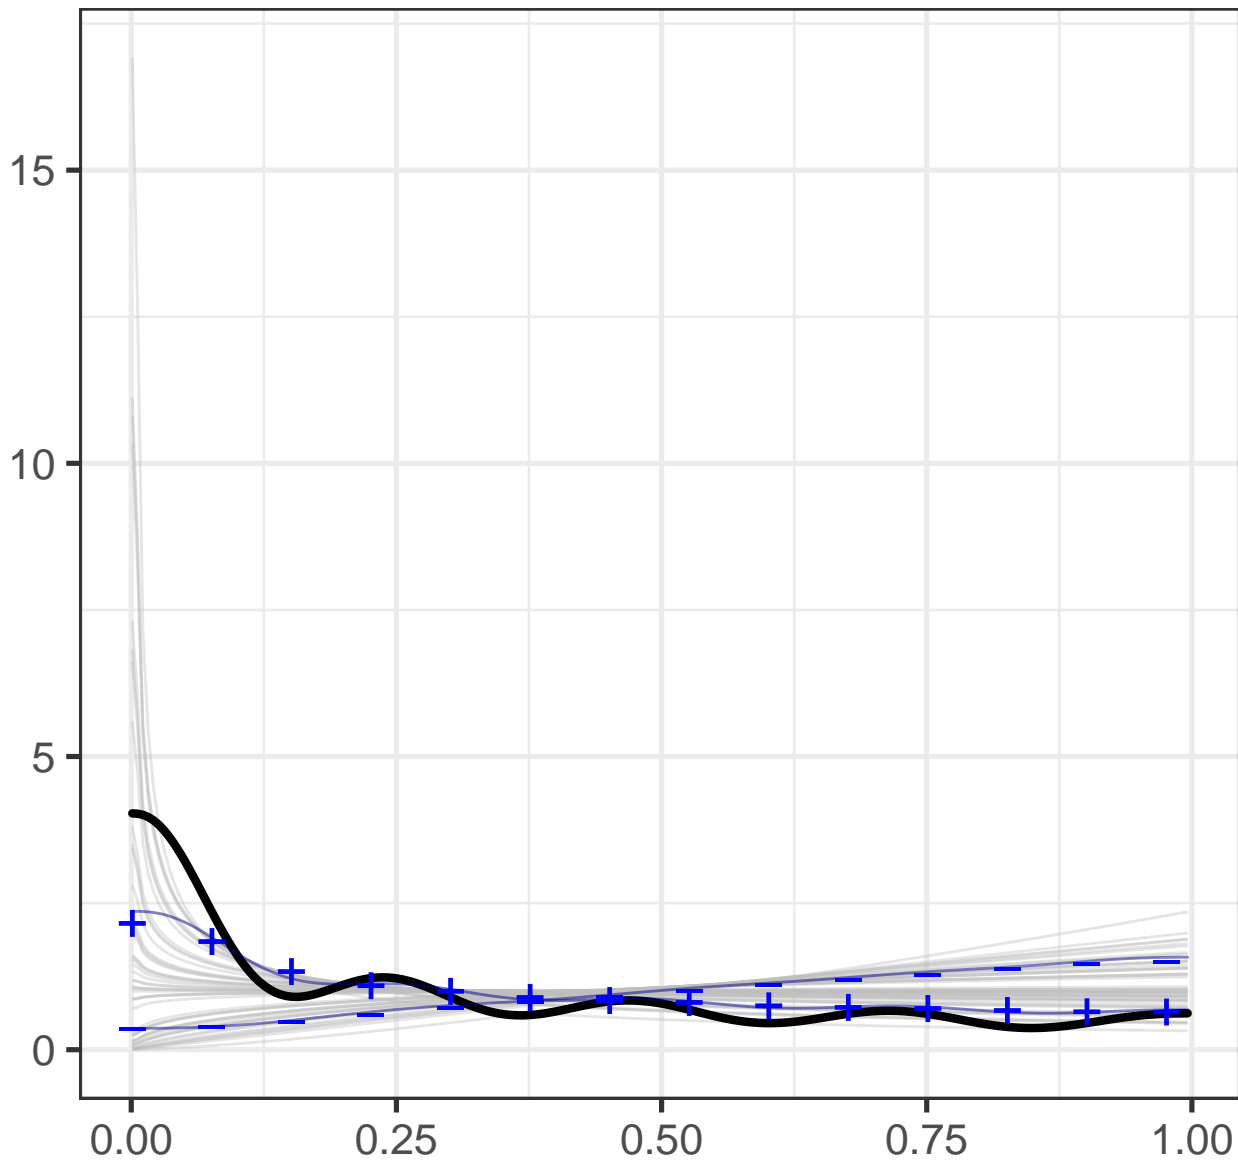

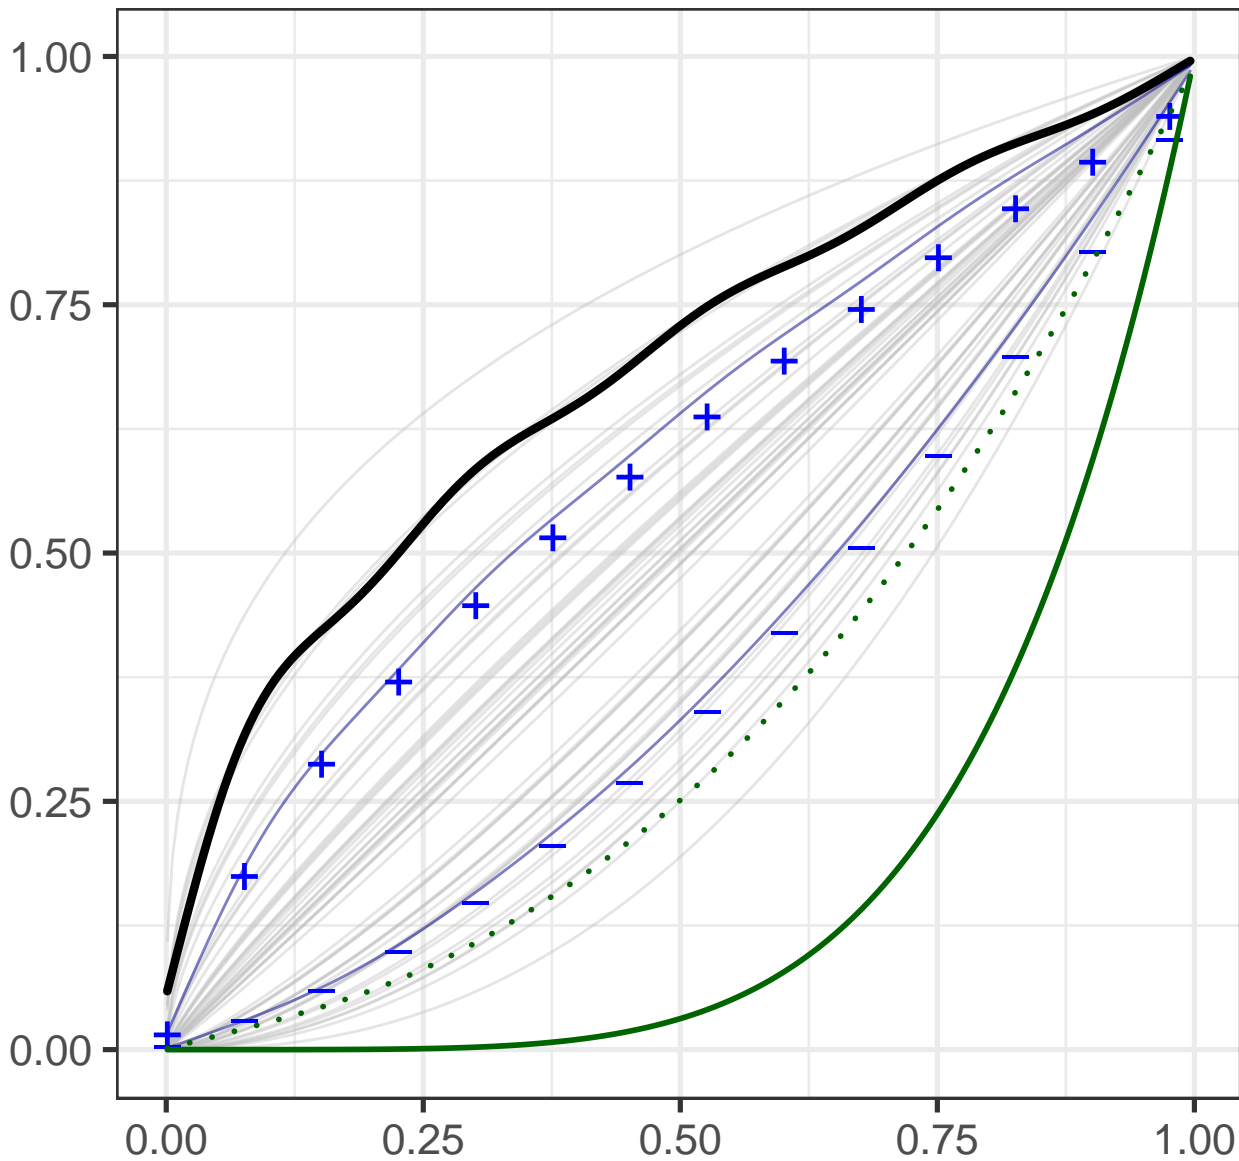

Supplement: Supplementary file 2 [file counterexample_Plots.pdf]
